# Supplementary material for: Large Language Model-Driven Cooperative Operator Ensemble Evolution for Permutation Flow Shop Scheduling
Source: arXiv:2606.15334 source file (2026-11-20)
Supplement: Supplementary file 1 [file supplement.tex]

\documentclass[lettersize,journal,onecolumn]{IEEEtran}

\usepackage{amsmath,amsfonts}
\usepackage{algorithmic}
\usepackage{algorithm}
\usepackage{array}
\usepackage[caption=false,font=normalsize,labelfont=sf,textfont=sf]{subfig}
\usepackage{textcomp}
\usepackage{stfloats}
\usepackage{url}
\usepackage{verbatim}
\usepackage{graphicx}
\usepackage{cite}
\usepackage{float}
\usepackage[hidelinks]{hyperref}
\usepackage{booktabs}
\usepackage{threeparttable}
\usepackage{xcolor}
\usepackage{capt-of}

\makeatletter
\renewcommand\subsubsection{\@startsection{subsubsection}{3}{\z@}%
  {-1.0ex \@plus -0.2ex \@minus -0.2ex}%
  {0.6ex \@plus 0.2ex}%
  {\normalfont\normalsize}}
\makeatother

\begin{document}

\title{Supplementary for the paper ``Large Language Model-Driven Cooperative Operator Ensemble Evolution for Permutation Flow Shop Scheduling''}

\maketitle

\subsection{The Iterated Greedy (IG) Algorithm}
\label{alg:ig_v0} 
The detailed procedure of the IG algorithm proposed by Ruiz and Stützle is presented in Algorithm~\ref{alg:ig}.

\begin{algorithm}[H]
\caption{The Iterated Greedy (IG) Algorithm}
\label{alg:ig}
\begin{algorithmic}[1]
\STATE \textbf{Input:} Destruction size $d$, Temperature factor $t$.
\STATE \textbf{Output:} Global best permutation $\pi^*$.
\STATE \textit{// Initialization using NEH algorithm}
\STATE $\pi \leftarrow \text{initialSolution}()$
\STATE \textit{// Apply local search to the initial solution}
\STATE $\pi \leftarrow \text{LocalSearch}(\pi)$
\STATE $\pi^* \leftarrow \pi$
\WHILE{termination criterion not met}
    \STATE \textit{// Remove $d$ jobs to form partial sequence}
    \STATE $(\pi_D, \pi_R) \leftarrow Destruction(\pi, d)$.
    \STATE \textit{// Insert removed jobs into best positions}
    \STATE $\pi' \leftarrow Construction(\pi_D, \pi_R)$.
    \STATE \textit{// Local Search phase}
    \STATE $\pi' \leftarrow LocalSearch(\pi')$.
    \STATE \textit{// Metropolis-based Acceptance Mechanism}
    \IF{$\text{Accept}(\pi', \pi, t)$}
        \STATE $\pi \gets \pi'$
    \ENDIF
    \STATE \textit{// Update global best solution}
    \IF{$C_{\max}(\pi) < C_{\max}(\pi^*)$}
        \STATE $\pi^* \gets \pi$ 
    \ENDIF
\ENDWHILE
\STATE \textbf{return} $\pi^*$ 
\end{algorithmic}
\end{algorithm}

\subsection{NEH Initialization and Local Search}
\label{alg:nehls} 
The NEH heuristic is commonly adopted to generate an initial job permutation for the permutation flow shop scheduling problem. Algorithm \ref{alg:neh} presents the detailed procedure of this initialization method.

\begin{algorithm}[H]
    \caption{NEH Initialization}
    \label{alg:neh}
    \begin{algorithmic}[1]
    \STATE \textbf{Input:} Processing times $P = \{p_{ij}\}$, number of jobs $n$, number of machines $m$
    \STATE \textbf{Output:} Initial solution $\pi$
    
    \STATE $\pi \leftarrow \emptyset$
    \STATE $\Pi^S \leftarrow$ jobs sorted in descending order of $\sum_{i=1}^{m} p_{ij}$ \hfill // larger total time first
    \STATE $\pi \leftarrow (\pi_1)$ \hfill // first job as initial sequence
    \STATE $\Pi^S \leftarrow \Pi^S \setminus \{\pi_1\}$
    \WHILE{$\Pi^S \neq \emptyset$}
        \STATE Select next job $\pi_1$ from $\Pi^S$
        \STATE $k^* \leftarrow \arg\min_{k \in \{1,\dots,|\pi|+1\}} C_{\max}(\text{insert}(\pi,\pi_1,k))$ \hfill // best position for min makespan
        \STATE $\pi \leftarrow \text{insert}(\pi,\pi_1,k^*)$
        \STATE $\Pi^S \leftarrow \Pi^S \setminus \{\pi_1\}$
    \ENDWHILE
    
    \STATE \textbf{return} $\pi$
    \end{algorithmic}
    \end{algorithm}

The insertion-based local search is used to refine a given solution by re-inserting jobs into more promising positions. Algorithm \ref{alg:insertion_ls} presents the corresponding local search procedure.

\begin{algorithm}[H]
    \caption{Local Search}
    \label{alg:insertion_ls}
    \begin{algorithmic}[1]
    \STATE \textbf{Input:} Solution $\pi$
    \STATE \textbf{Output:} Solution $\pi$ and its makespan $C_{\max}(\pi)$
    \STATE $C_{\max}^* \leftarrow C_{\max}(\pi)$ \hfill // current best makespan
    \FOR{$i = 1$ \textbf{to} $|\pi|$} 
        \STATE $job \leftarrow \pi[i]$; remove $job$ from $\pi$
        \STATE $k^* \leftarrow \arg\min_{k \in \{1,\dots,|\pi|+1\}} C_{\max}(\text{insert}(\pi, job, k))$ \hfill // best insertion position
        \STATE $\pi \leftarrow \text{insert}(\pi, job, k^*)$
        \IF{$C_{\max}(\pi) < C_{\max}^*$}
            \STATE \textbf{return} $\pi$, $C_{\max}(\pi)$ \hfill // first improvement, return immediately
        \ENDIF
        \STATE $C_{\max}^* \leftarrow C_{\max}(\pi)$ 
    \ENDFOR
    \STATE \textbf{return} $\pi$, $C_{\max}^*$ 
    \end{algorithmic}
    \end{algorithm}

\subsection{Empirical Derivation of the Stagnation Threshold $\tau$}
\label{analyse_stagnation} 
To determine the stagnation threshold $\tau$ for the STSS mechanism, we conducted a comprehensive statistical analysis of the stagnation behaviors during the search process using $\text{IG}_{\text{ReEvo}}$. During the algorithmic execution, we recorded the historical sequence of the global best makespan. An improvement point is defined as any iteration where the global best solution strictly improves upon the previous best, with the initial solution at iteration 0 considered the first improvement point. Consequently, a stagnation period is defined as the number of iterations elapsed between two consecutive improvement points. This metric directly represents the duration the algorithm spends searching before finding a superior solution.

For each problem scale, we independently executed the algorithm 20 times and merged all generated stagnation periods into a single comprehensive sample pool. On this aggregated dataset, we calculated various percentiles, including the 75\%, 80\%, 85\%, 90\%, 95\%, and 99\%, using the nearest interpolation method. This specific interpolation approach was chosen to ensure that the resulting threshold remains strictly an integer, which aligns with the discrete nature of algorithmic iterations. The 99\% was ultimately selected as the reference threshold because it effectively captures the upper bound of the vast majority of productive explorations. In practical executions, approximately 99\% of productive stagnation periods do not exceed this value. By setting the switching trigger at this condition, the algorithm is granted sufficient time to fully exploit the current neighborhood and escape local optima, while strictly avoiding the accumulation of excessive invalid iterations once an operator has essentially stalled. As illustrated in Fig.~\ref{fig:threshold}, the observed 99\% values across different job scales ($n$) closely follow the empirical decay curve $\tau = \lfloor 1000 / \sqrt{n} \rfloor$.

Furthermore, our statistical observations indicated that the stagnation period, when measured in iterations, is overwhelmingly dominated by the number of jobs $n$. While the machine count $m$ affects the computational time required per evaluation, it does not show a significant or regular correlation with the required iteration lengths between consecutive improvements. Therefore, to preserve the simplicity and robustness of the control logic, the parameter $m$ is explicitly excluded from the threshold formulation.

\begin{figure}[H]
  \centering
  \includegraphics[width=0.8\linewidth]{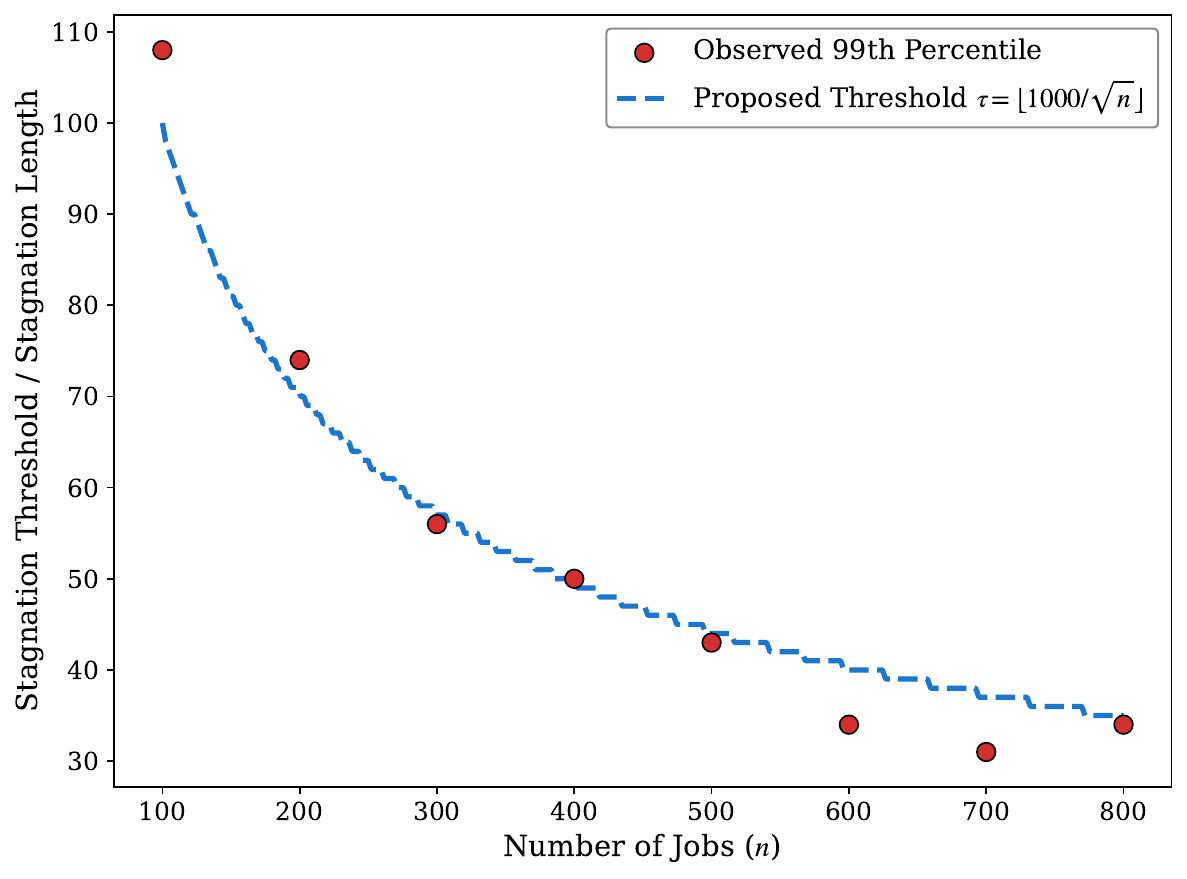} 
  \caption{Empirical 99th Percentile of Stagnation Lengths vs. Proposed Stagnation Threshold}
  \label{fig:threshold}
\end{figure}

\subsection{Prompts}
\label{prompts} 
The prompts adopted in the SCOE framework are reported in this subsection.
\subsubsection{System Prompt}
\begin{center}
  \includegraphics[width=\linewidth]{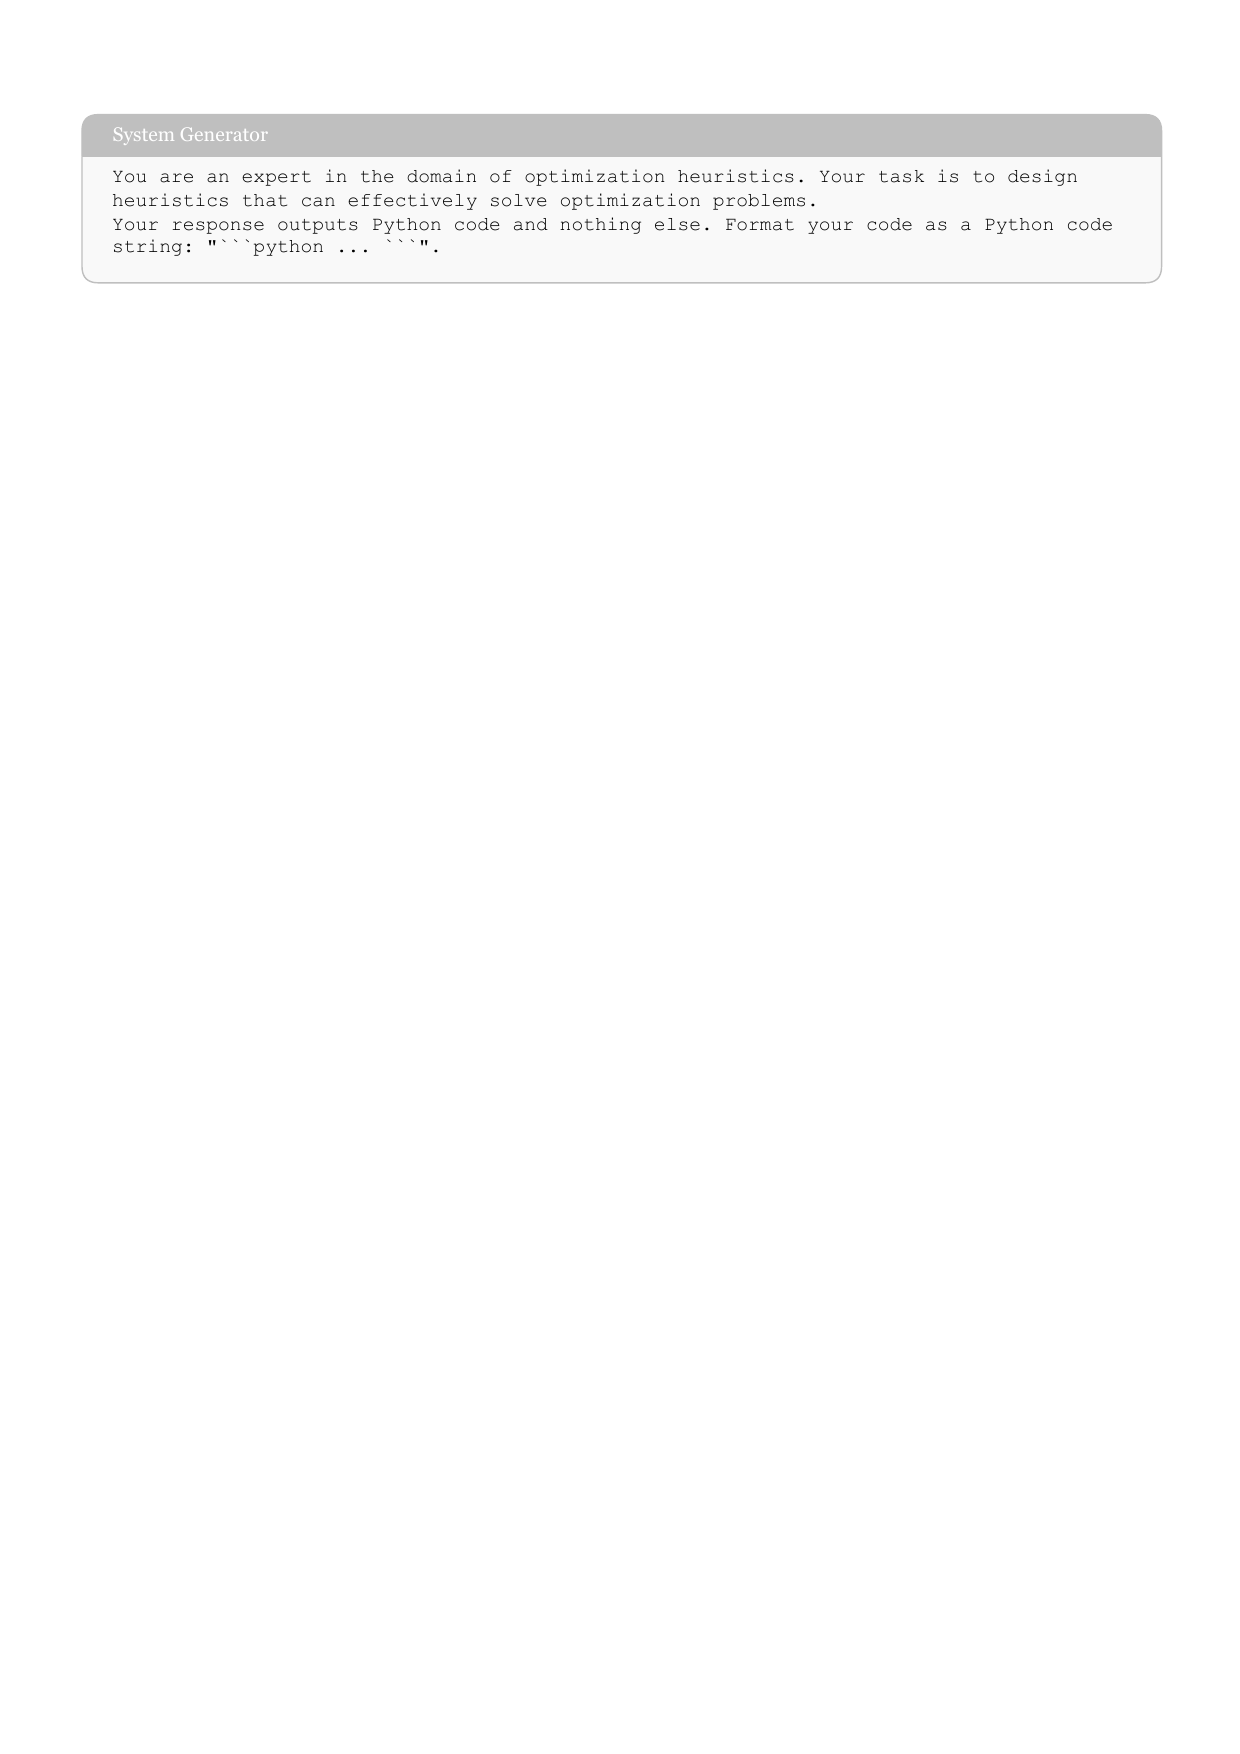}
  \vspace{0.5em}
  \text{Prompt 1: System prompt for generator LLM}
\end{center}

\begin{center}
  \includegraphics[width=\linewidth]{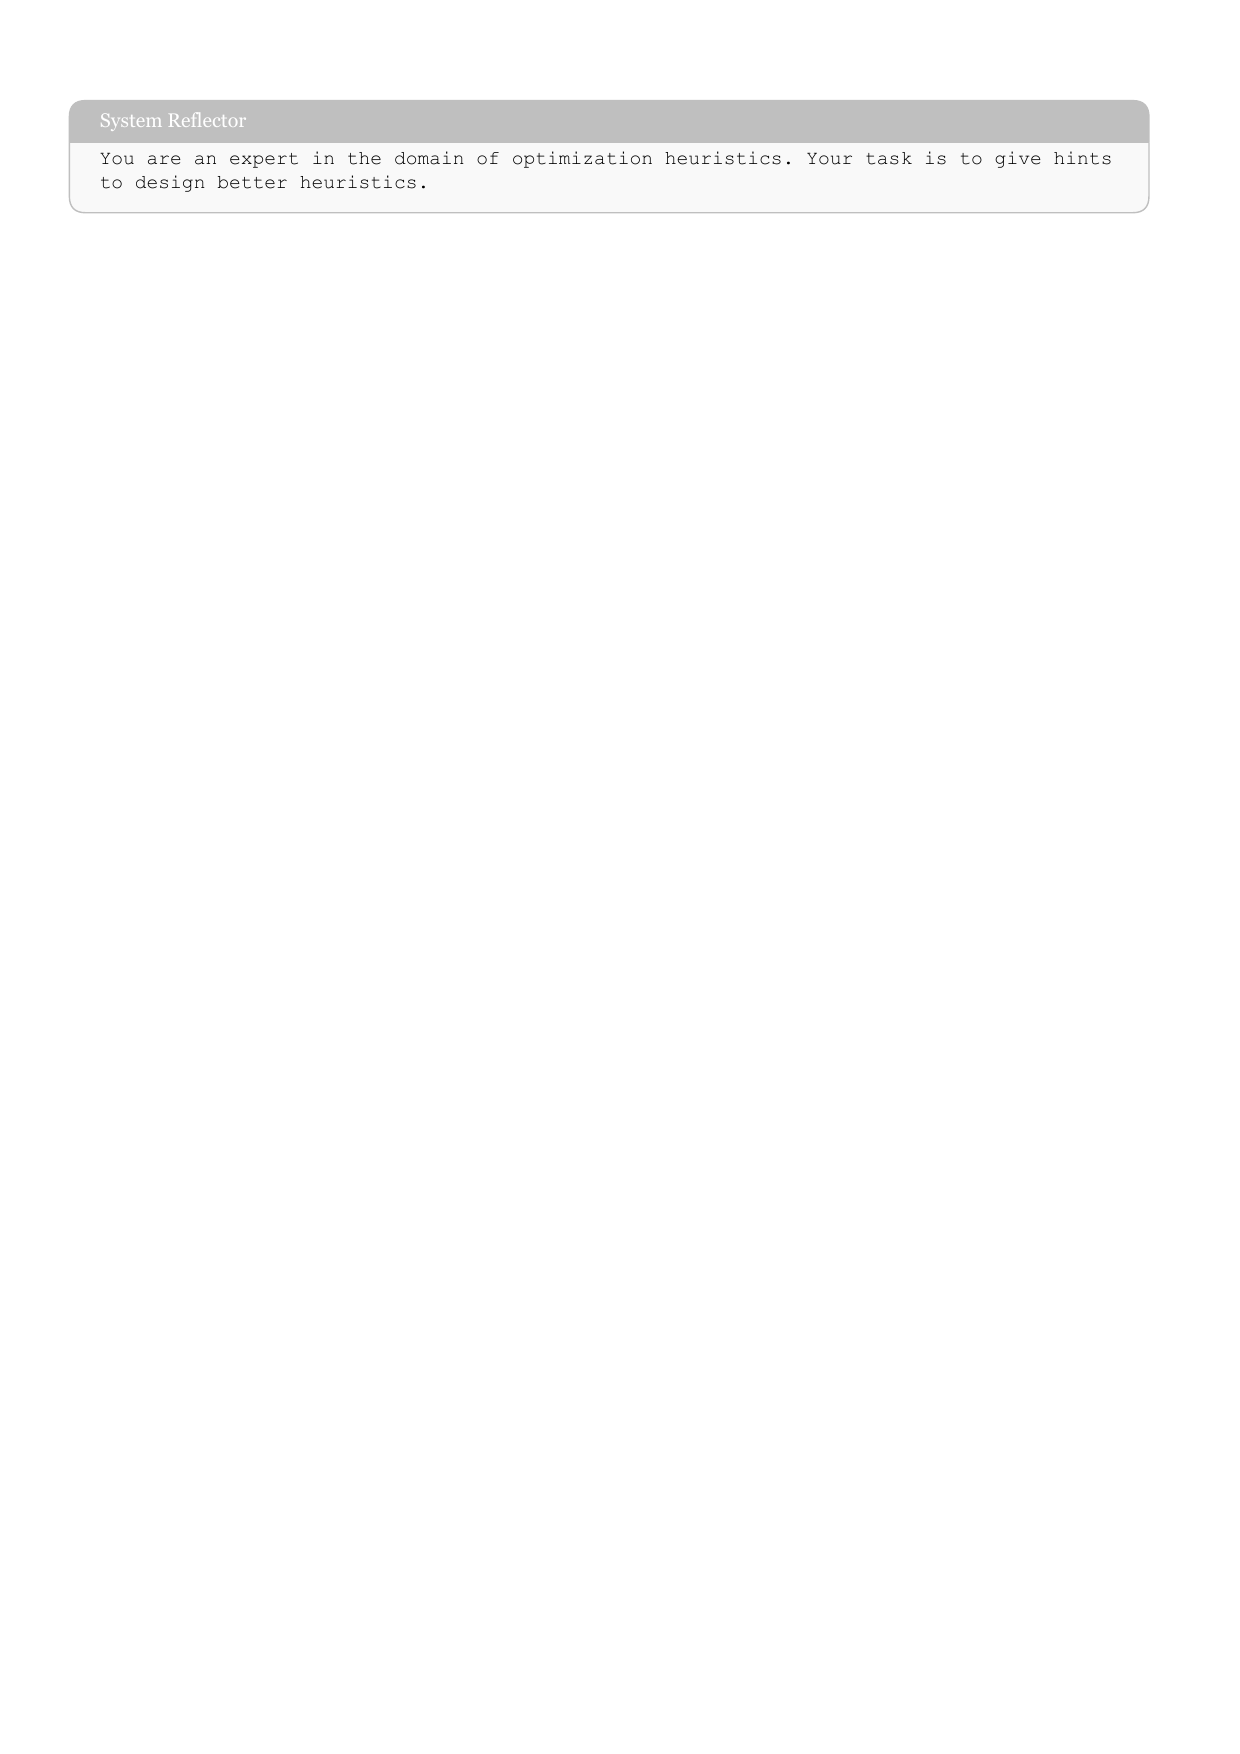}
  \vspace{0.5em}
  \text{Prompt 2: System prompt for reflector LLM}
\end{center}

\subsubsection{Generation Prompt}
\begin{center}
  \includegraphics[width=\linewidth]{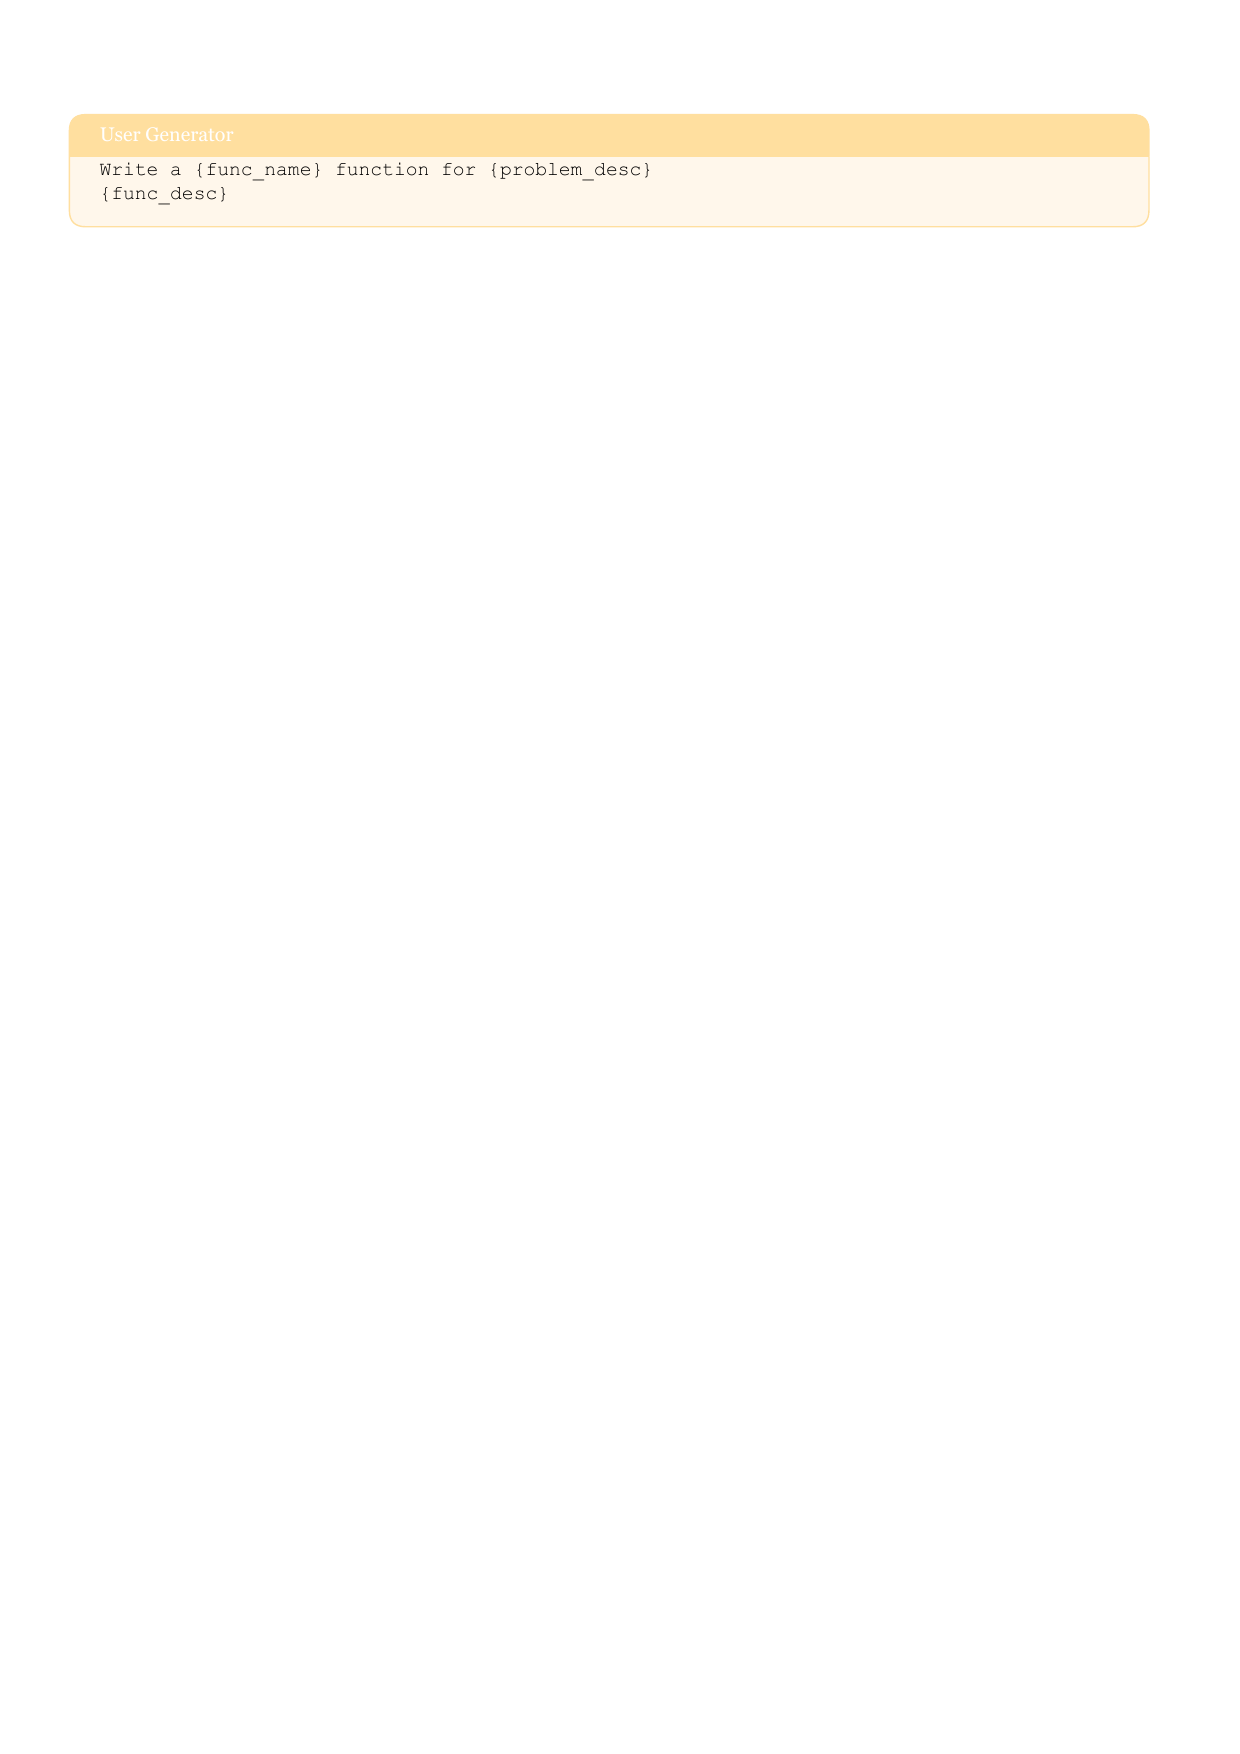}
  \vspace{0.5em}
  \text{Prompt 3: User prompt for target function generation}
\end{center}

\begin{center}
  \includegraphics[width=\linewidth]{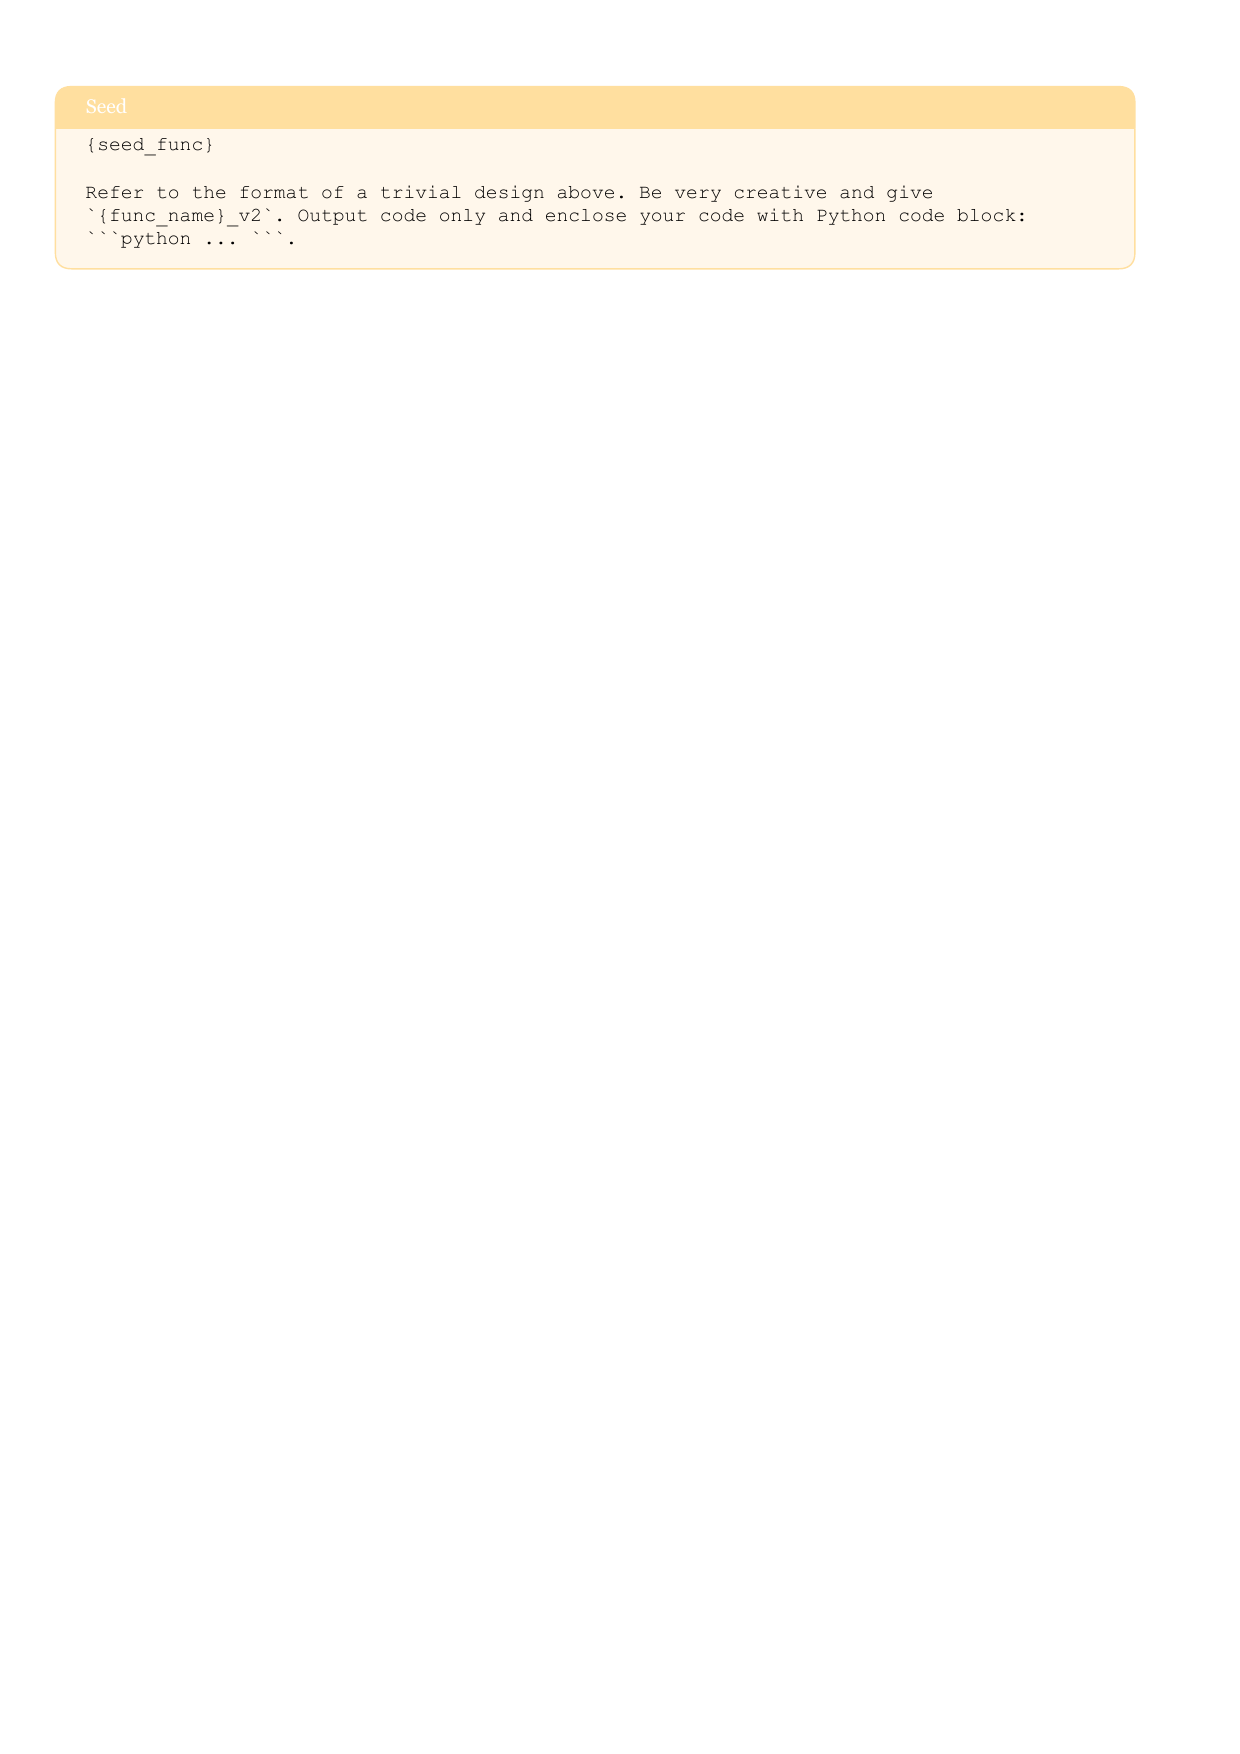}
  \vspace{0.5em}
  \text{Prompt 4: Seed format prompt}
\end{center}

\begin{center}
  \includegraphics[width=\linewidth]{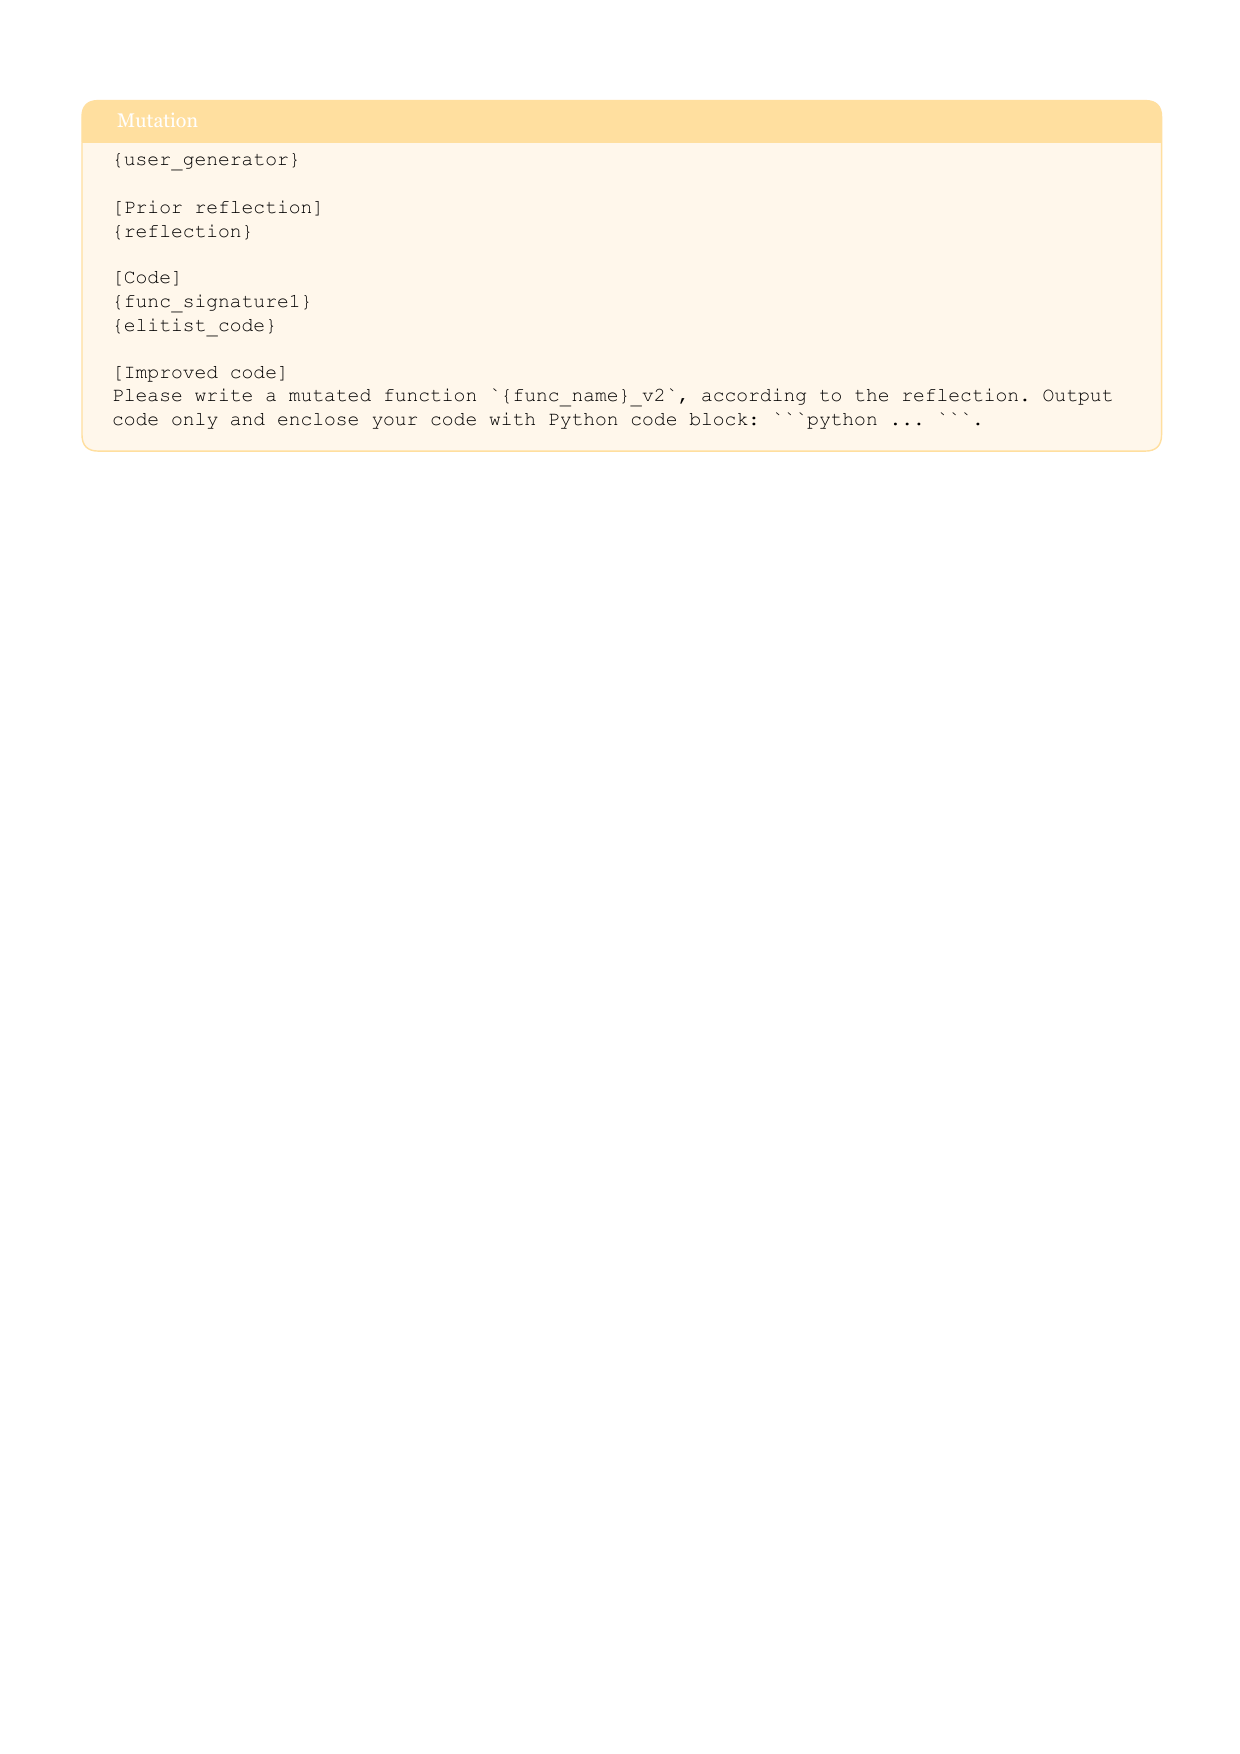}
  \vspace{0.5em}
  \text{Prompt 5: User prompt for mutation}
\end{center}

\begin{center}
  \includegraphics[width=\linewidth]{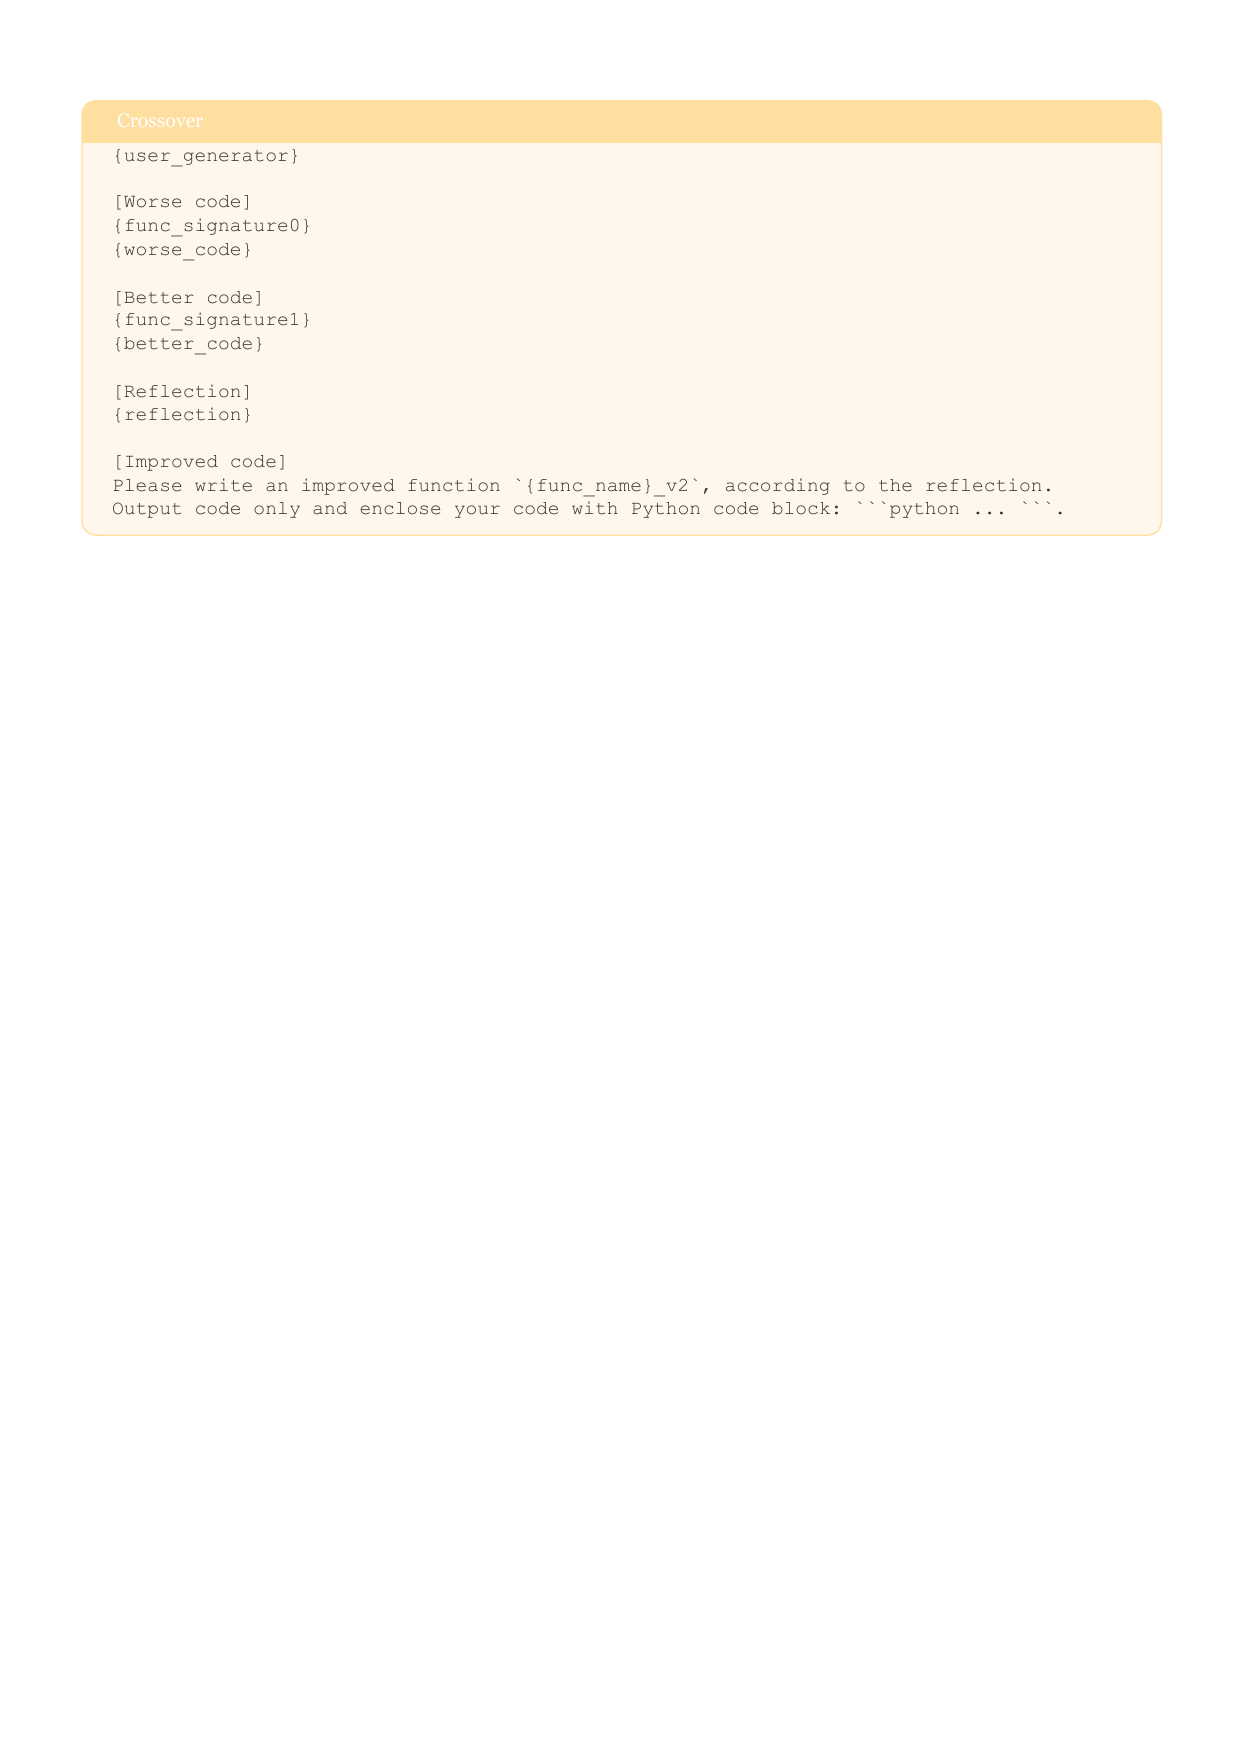}
  \vspace{0.5em}
  \text{Prompt 6: User prompt for crossover}
\end{center}

\subsubsection{Reflection Prompt}
\begin{center}
  \includegraphics[width=\linewidth]{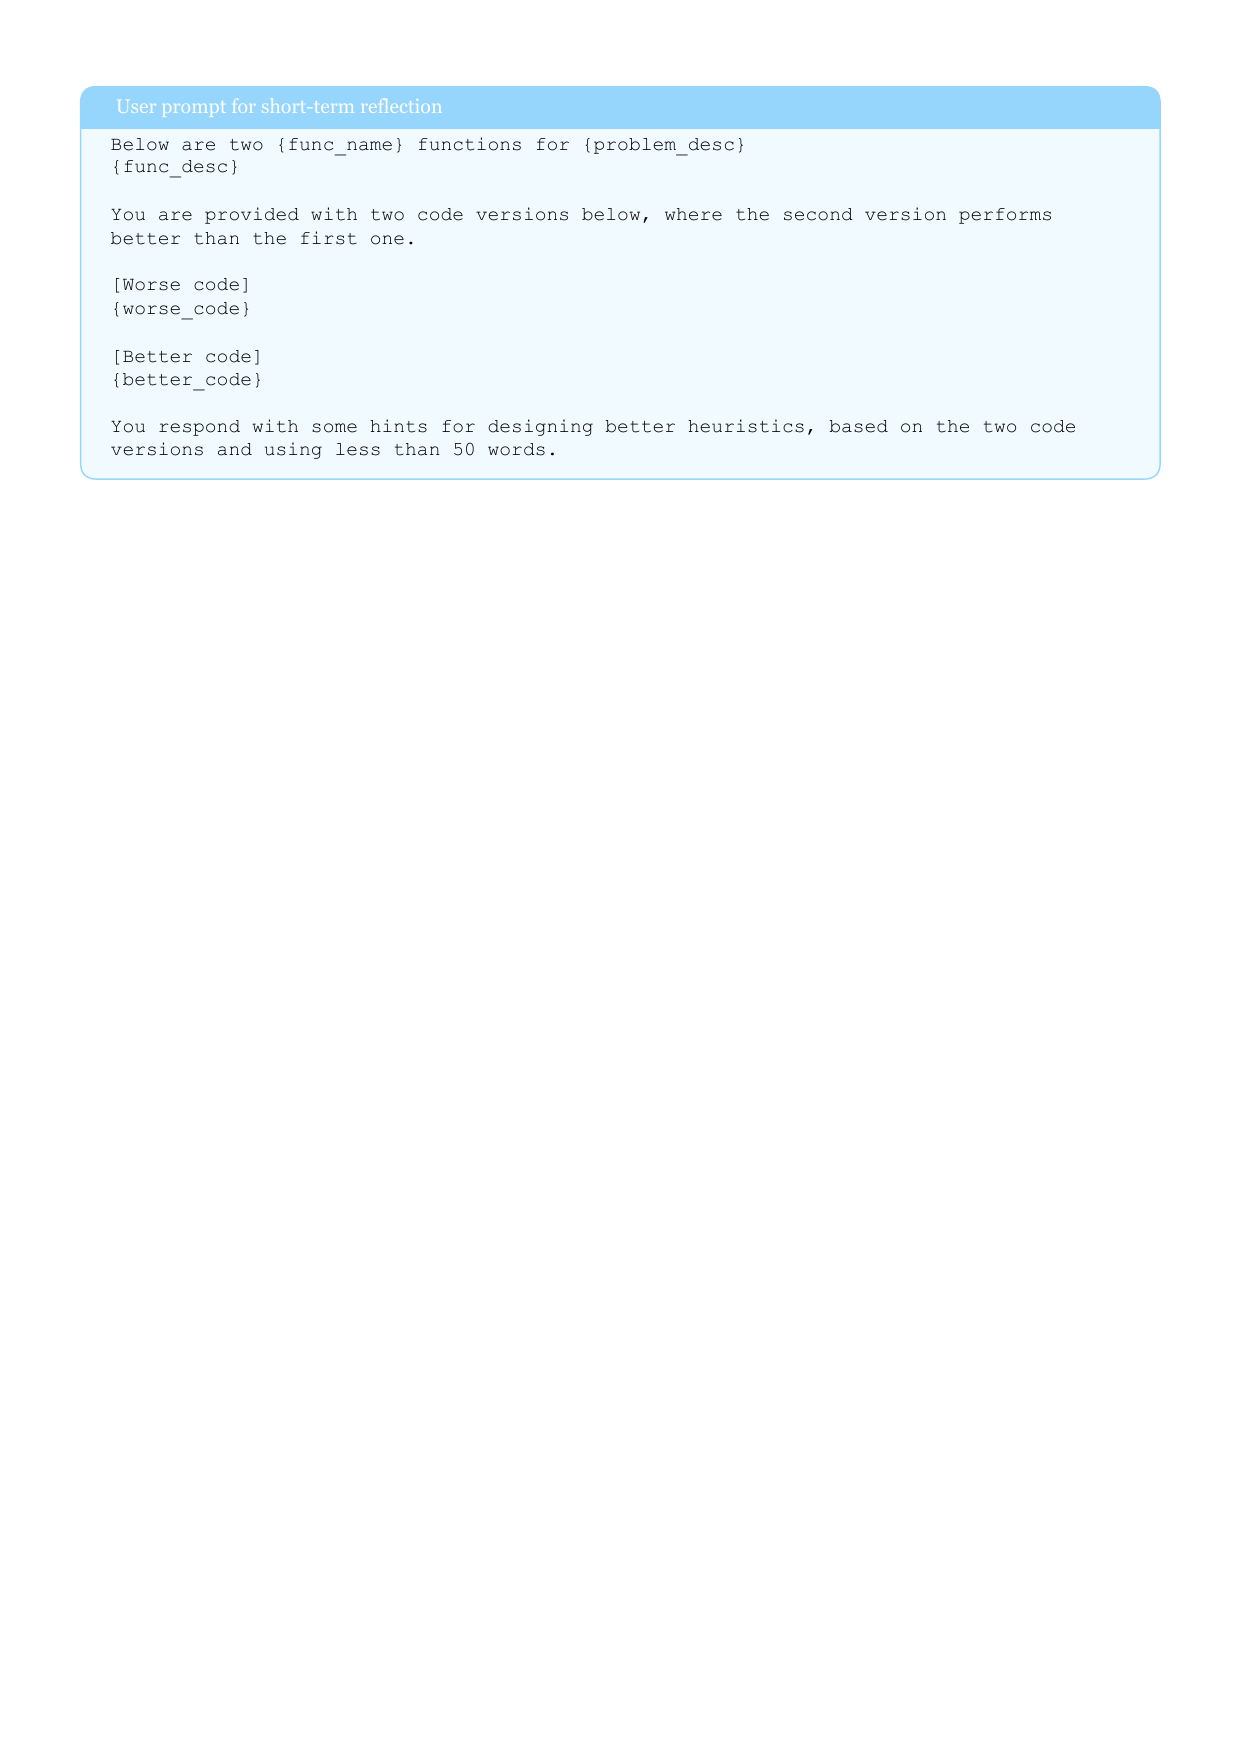}
  \vspace{0.5em}
  \text{Prompt 7: User prompt for short-term reflection}
\end{center}

\begin{center}
  \includegraphics[width=\linewidth]{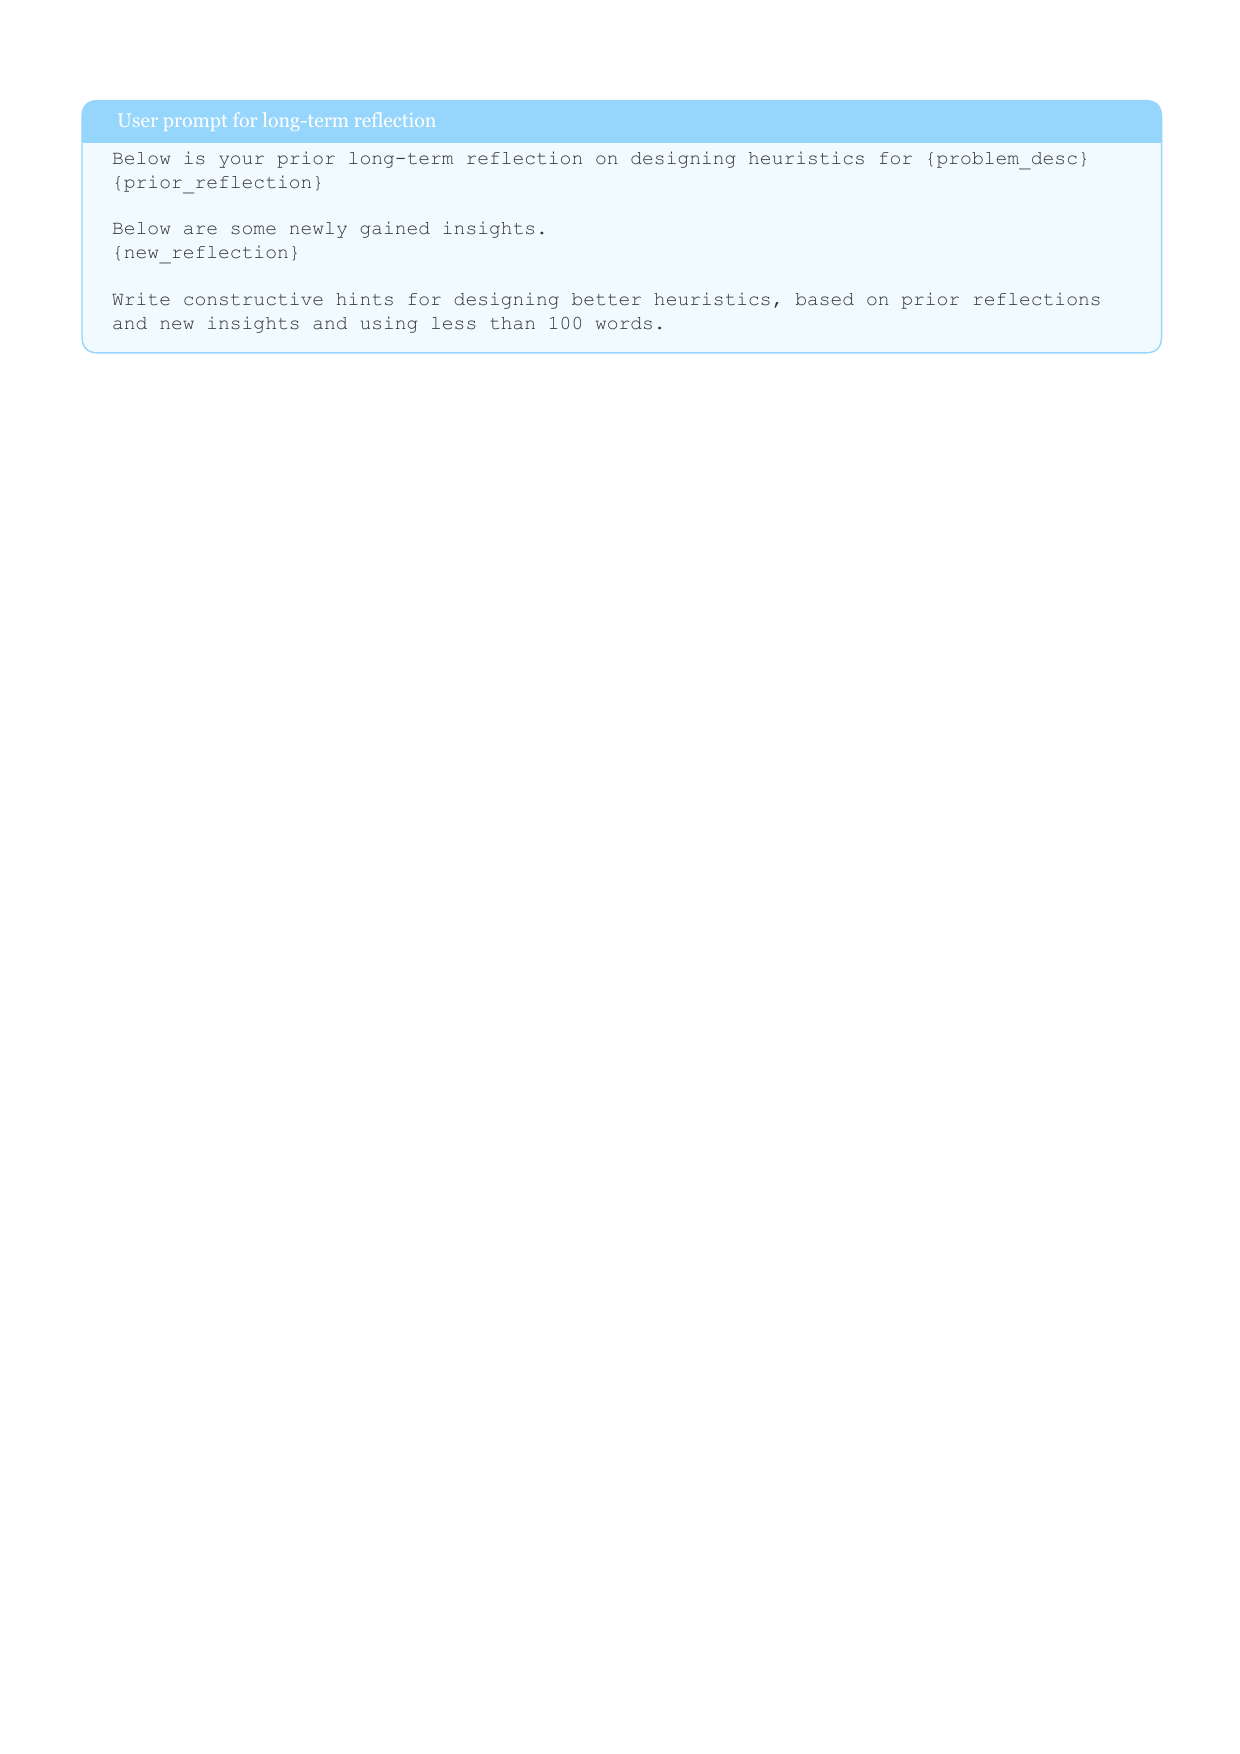}
  \vspace{0.5em}
  \text{Prompt 8: User prompt for long-term reflection}
\end{center}

\subsubsection{Operator Ensemble State-Awareness Prompt}
\begin{center}
  \includegraphics[width=\linewidth]{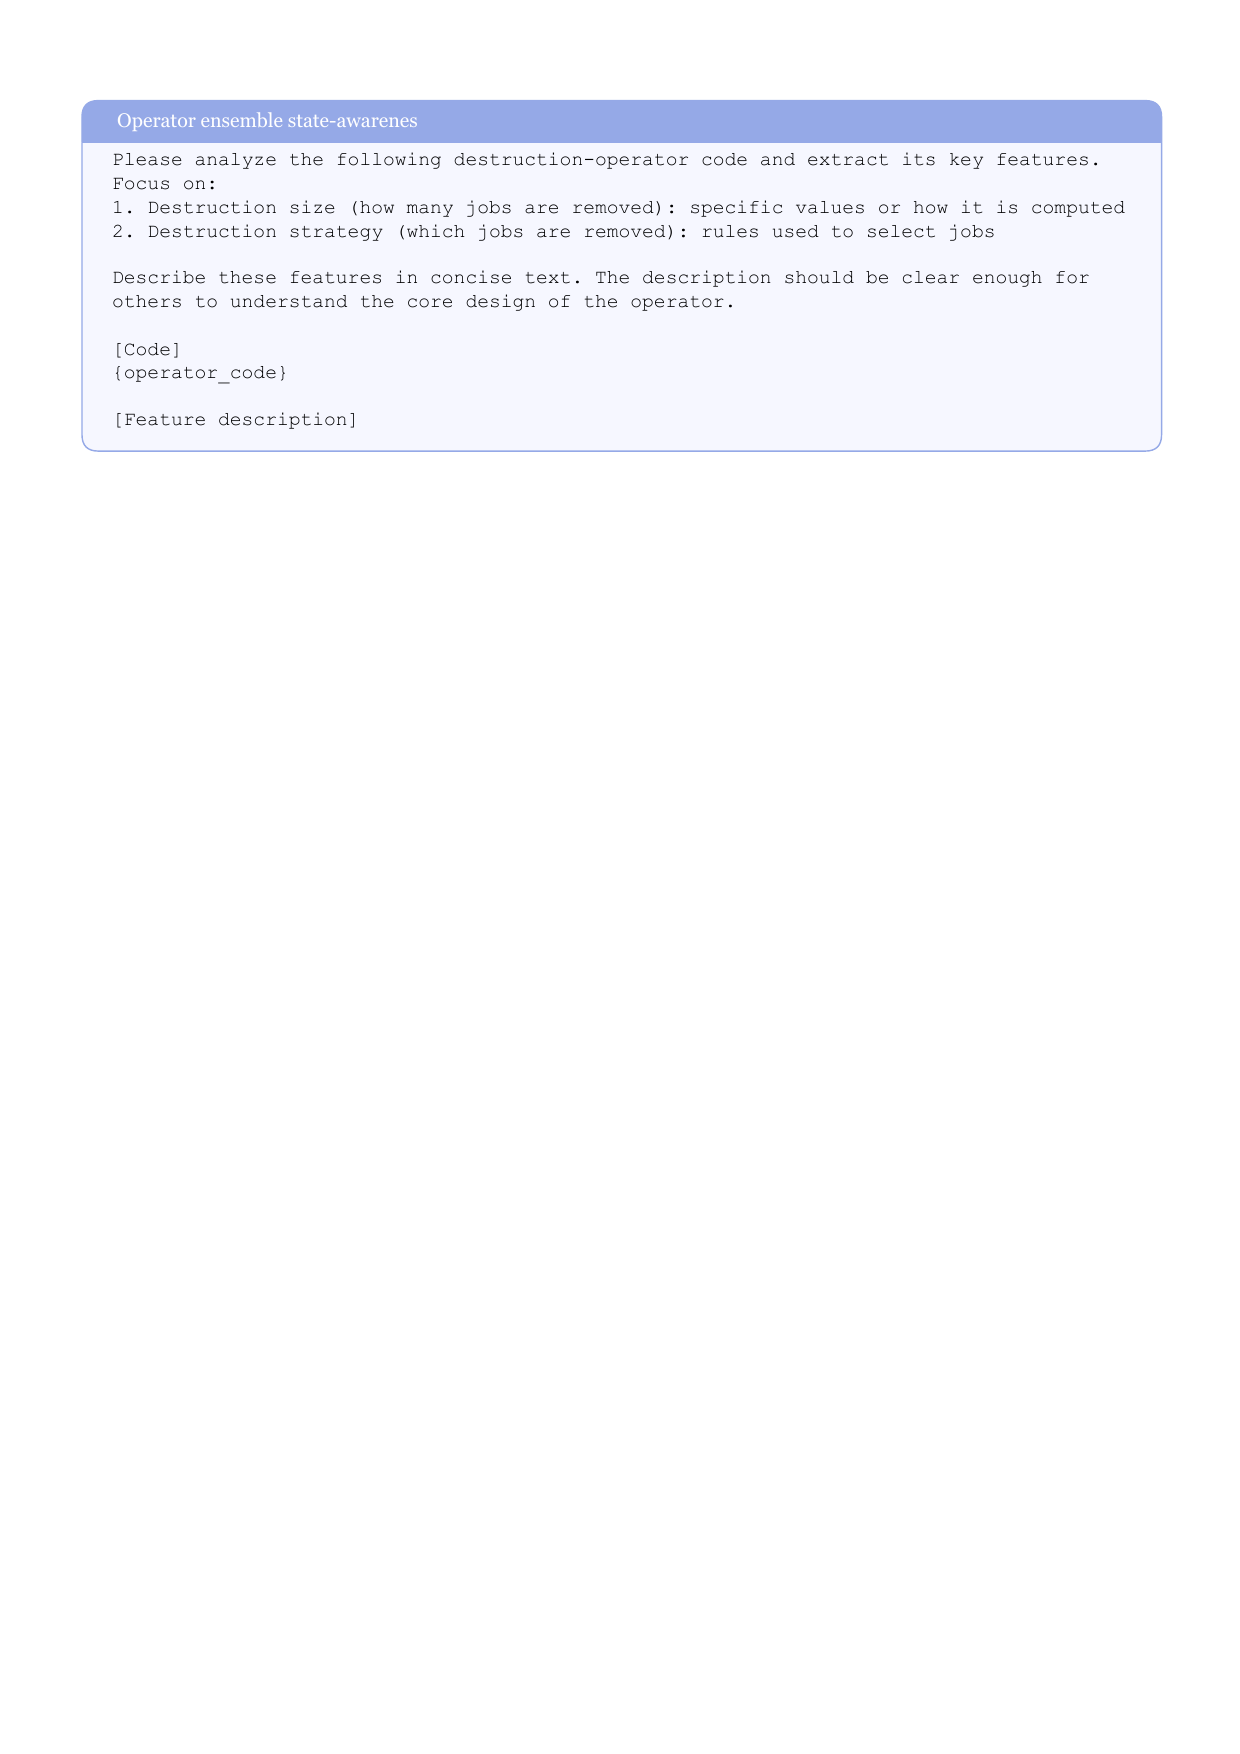}
  \vspace{0.5em}
  \text{Prompt 9: User prompt for state-aware}
\end{center}

\subsubsection{Task-Specific Prompts}
\begin{center}
  \includegraphics[width=\linewidth]{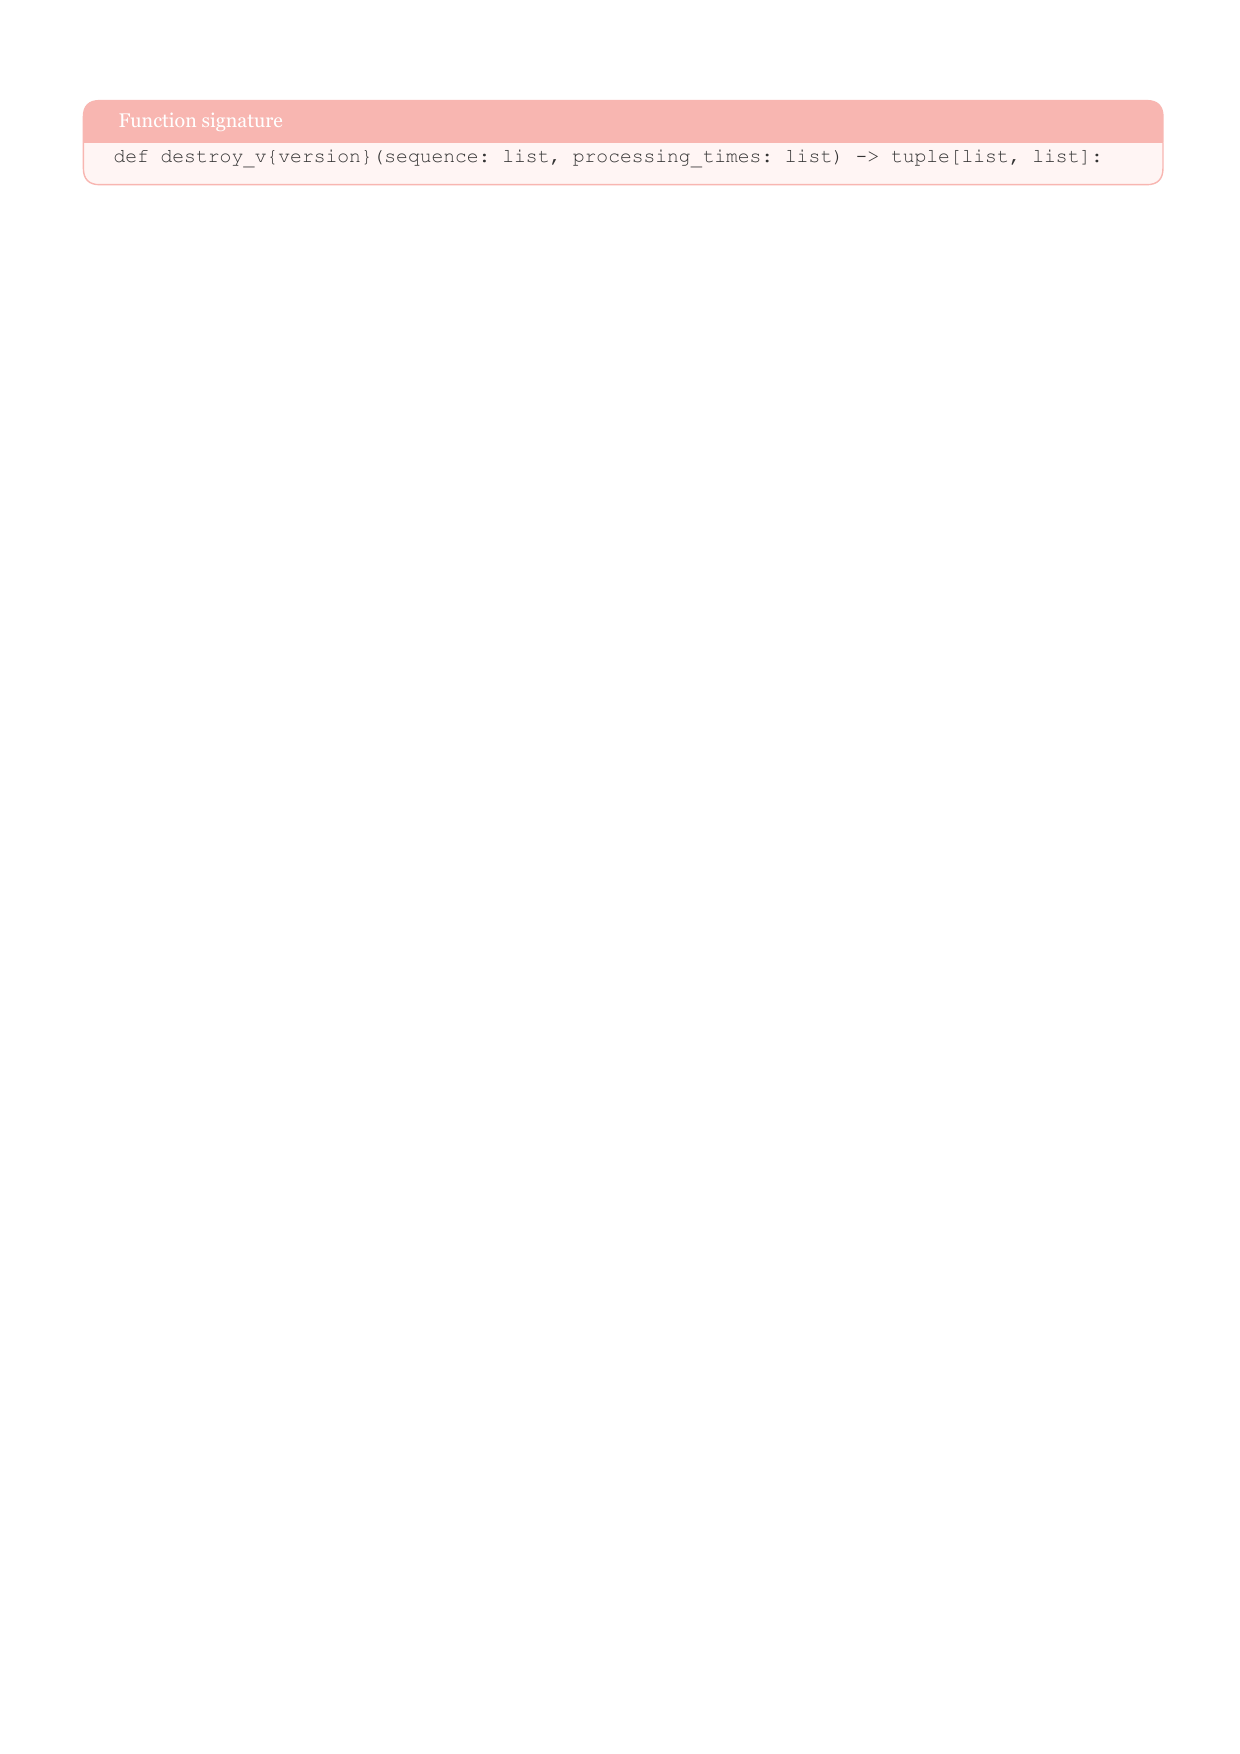}
  \vspace{0.5em}
  \text{Prompt 10: Operator signature}
\end{center}

\begin{center}
  \includegraphics[width=\linewidth]{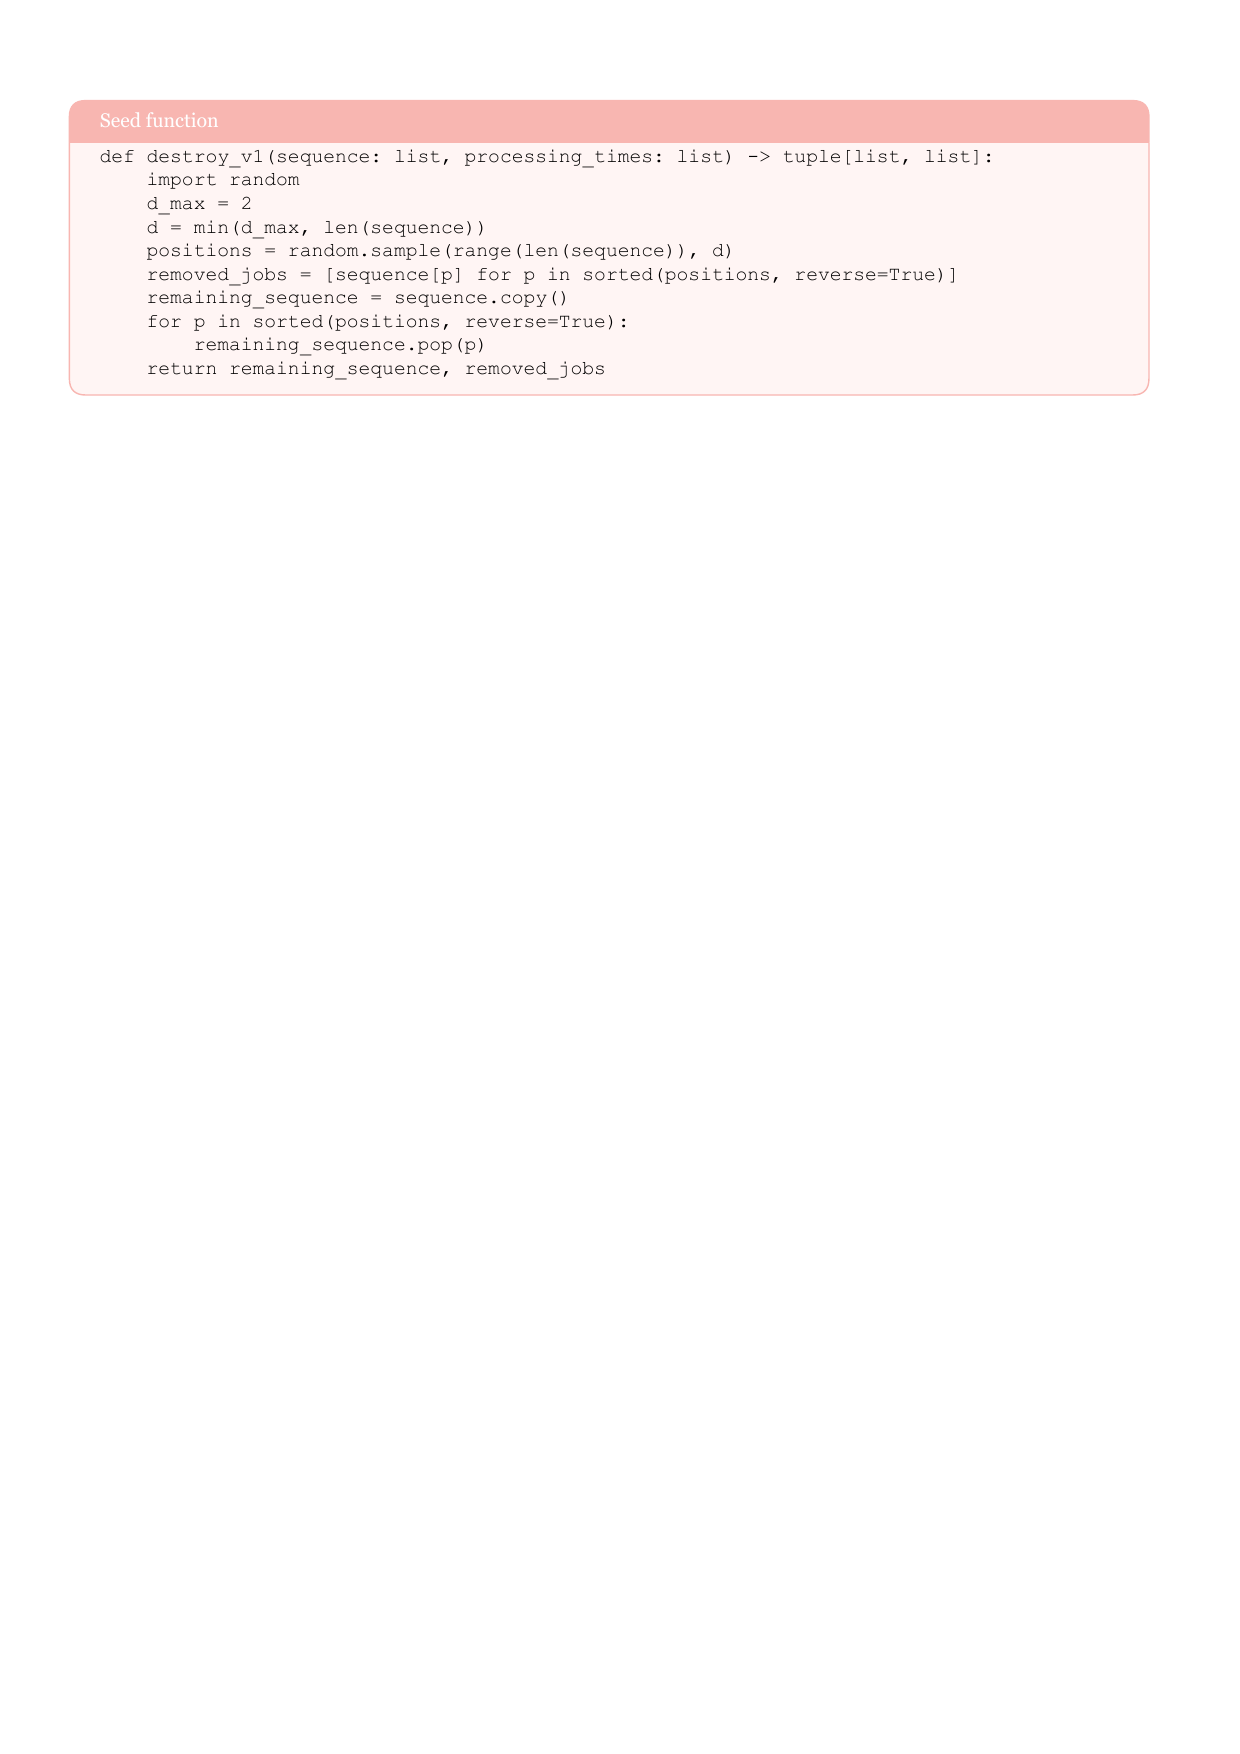}
  \vspace{0.5em}
  \text{Prompt 11: Seed operator}
\end{center}

\begin{center}
  \includegraphics[width=\linewidth]{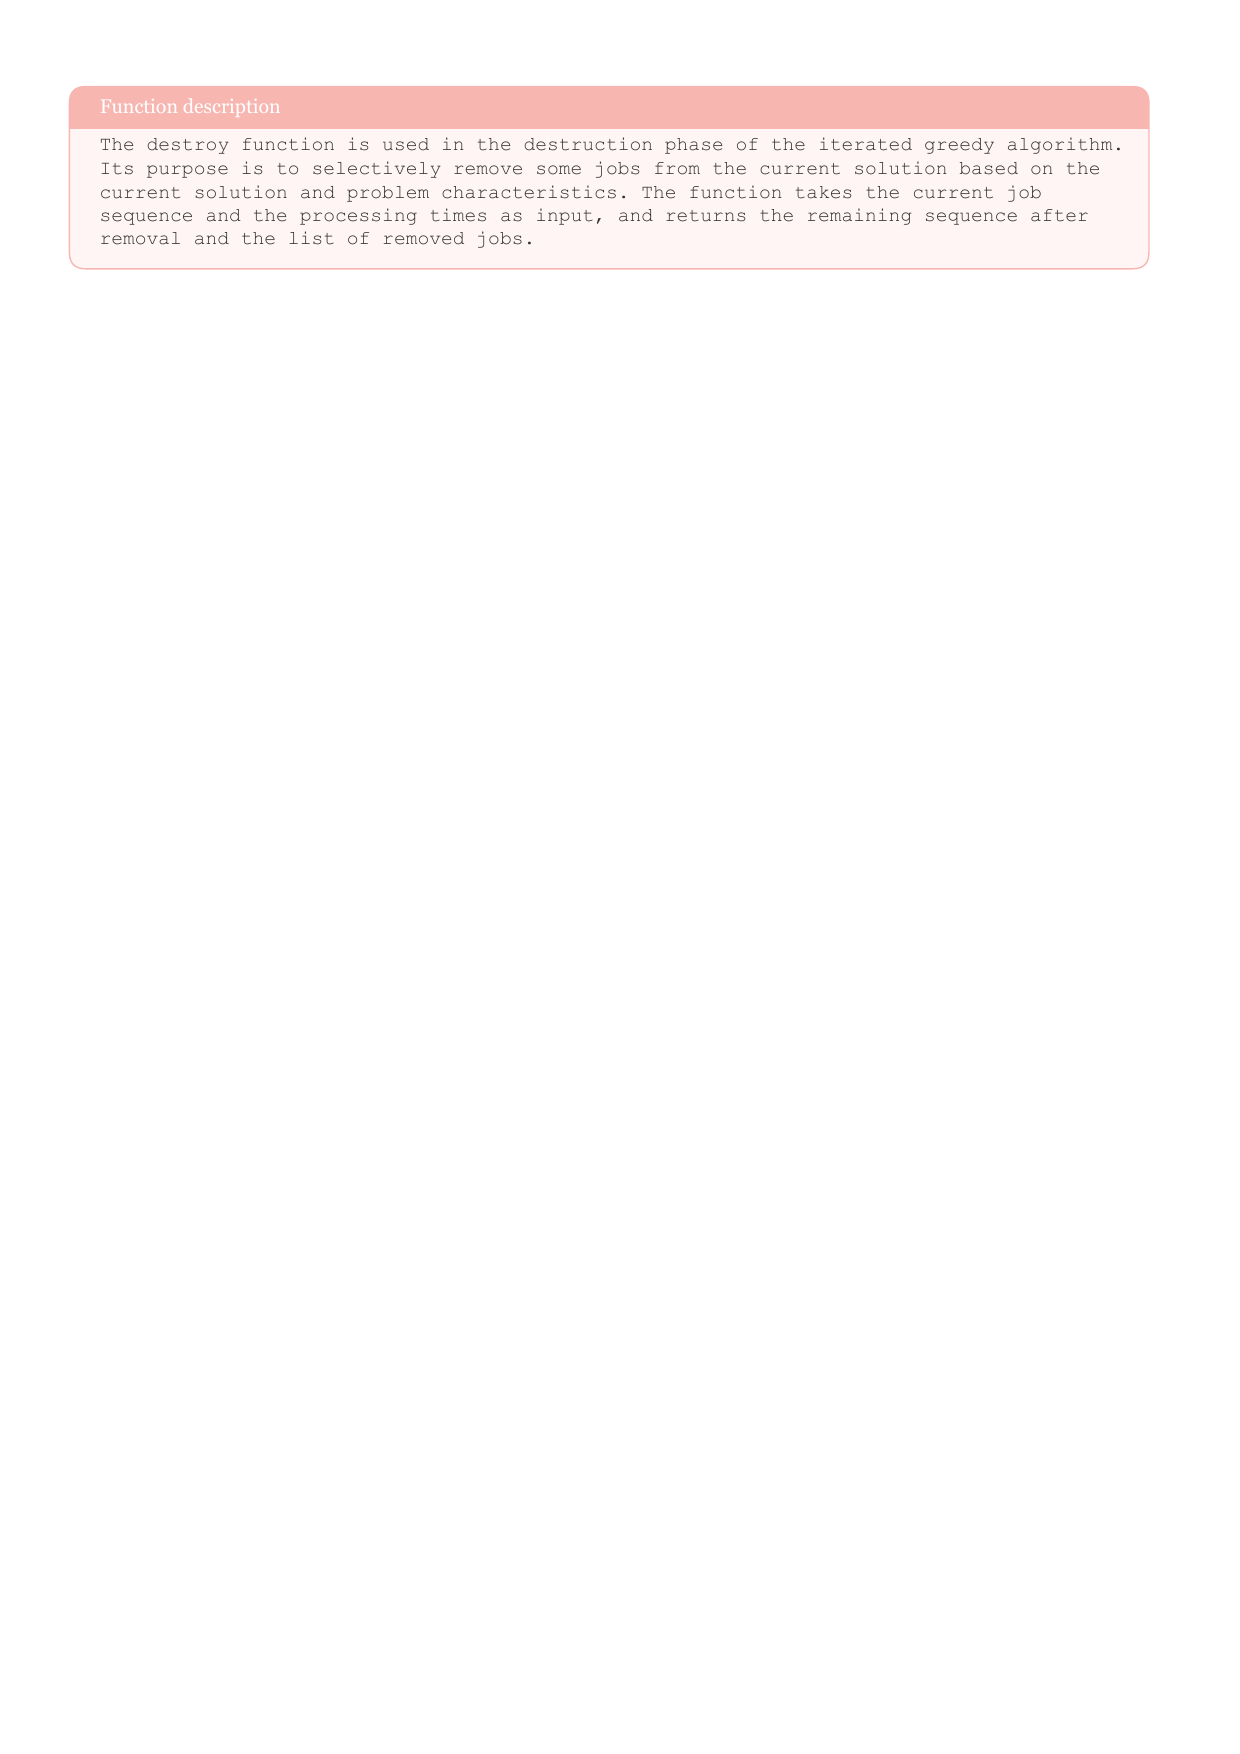}
  \vspace{0.5em}
  \text{Prompt 12: Operator description}
\end{center}

\begin{center}
  \includegraphics[width=\linewidth]{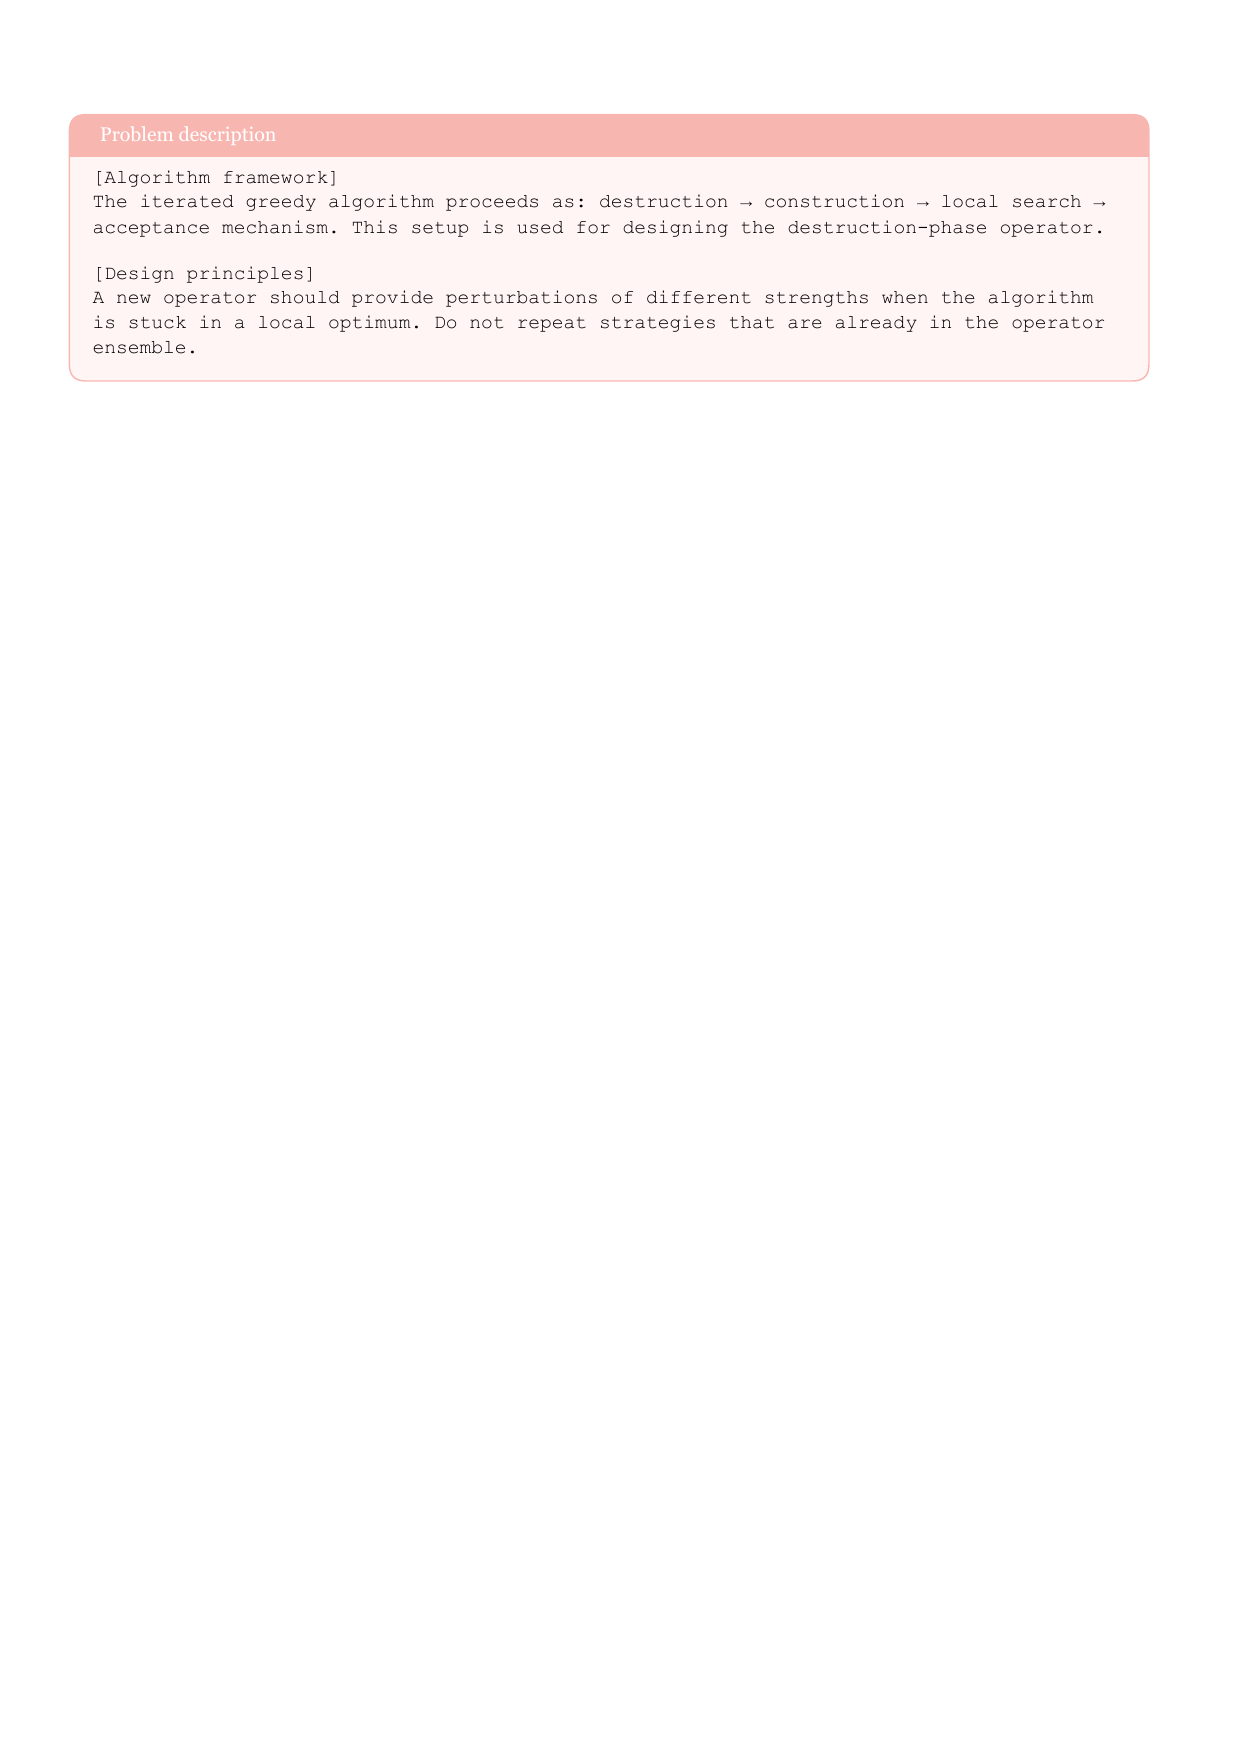}
  \vspace{0.5em}
  \text{Prompt 13: Domain knowledge}
\end{center}

\subsection{Parameters of Co-ReEvo}
\label{reevo_params} 
The parameter settings of Co-ReEvo used in this study are presented in Table~\ref{tab:params}.

\begin{table}[h!]
    \centering
    \caption{Parameter Settings of Co-ReEvo}
    \label{tab:params}
    \begin{tabular}{l|c}
        \toprule
        Parameter & Value \\
        \midrule
        LLM temperature (generator and reflector) & 1 \\
        Population size & 10 \\
        Number of initial generations & 30\\
        Maximum number of evaluations & 76 \\
        Crossover rate & 1 \\
        Mutation rate & 0.5 \\
        \bottomrule
    \end{tabular}
\end{table}

\subsection{Generated Destruction Operators Ensemble}
\label{code} 
This subsection presents the four destruction operators evolved by SCOE with Qwen2.5-Max.
These operators are integrated into IG-DOE.
\begin{center}
  \includegraphics[width=\linewidth]{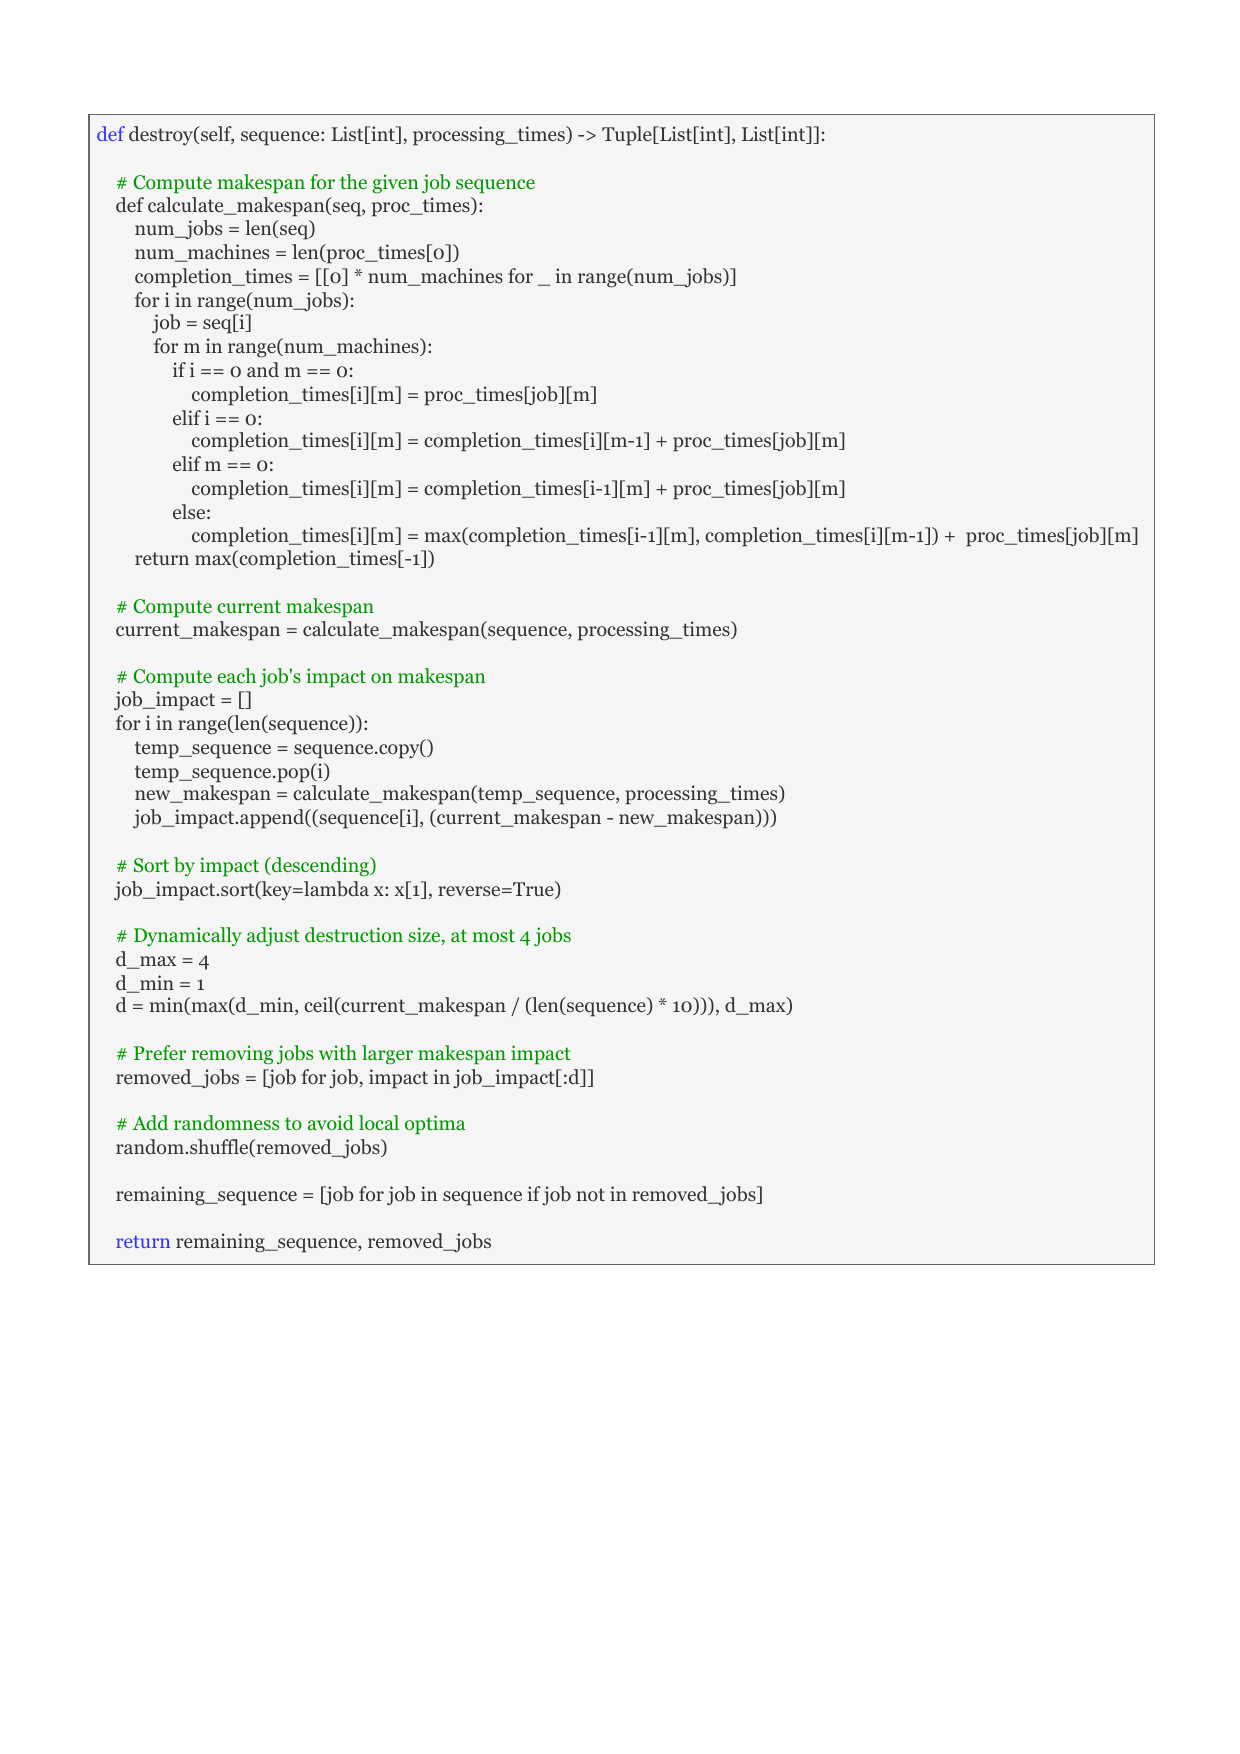}
  \vspace{0.5em}
  \text{Operator1}
\end{center}

\begin{center}
  \includegraphics[width=\linewidth]{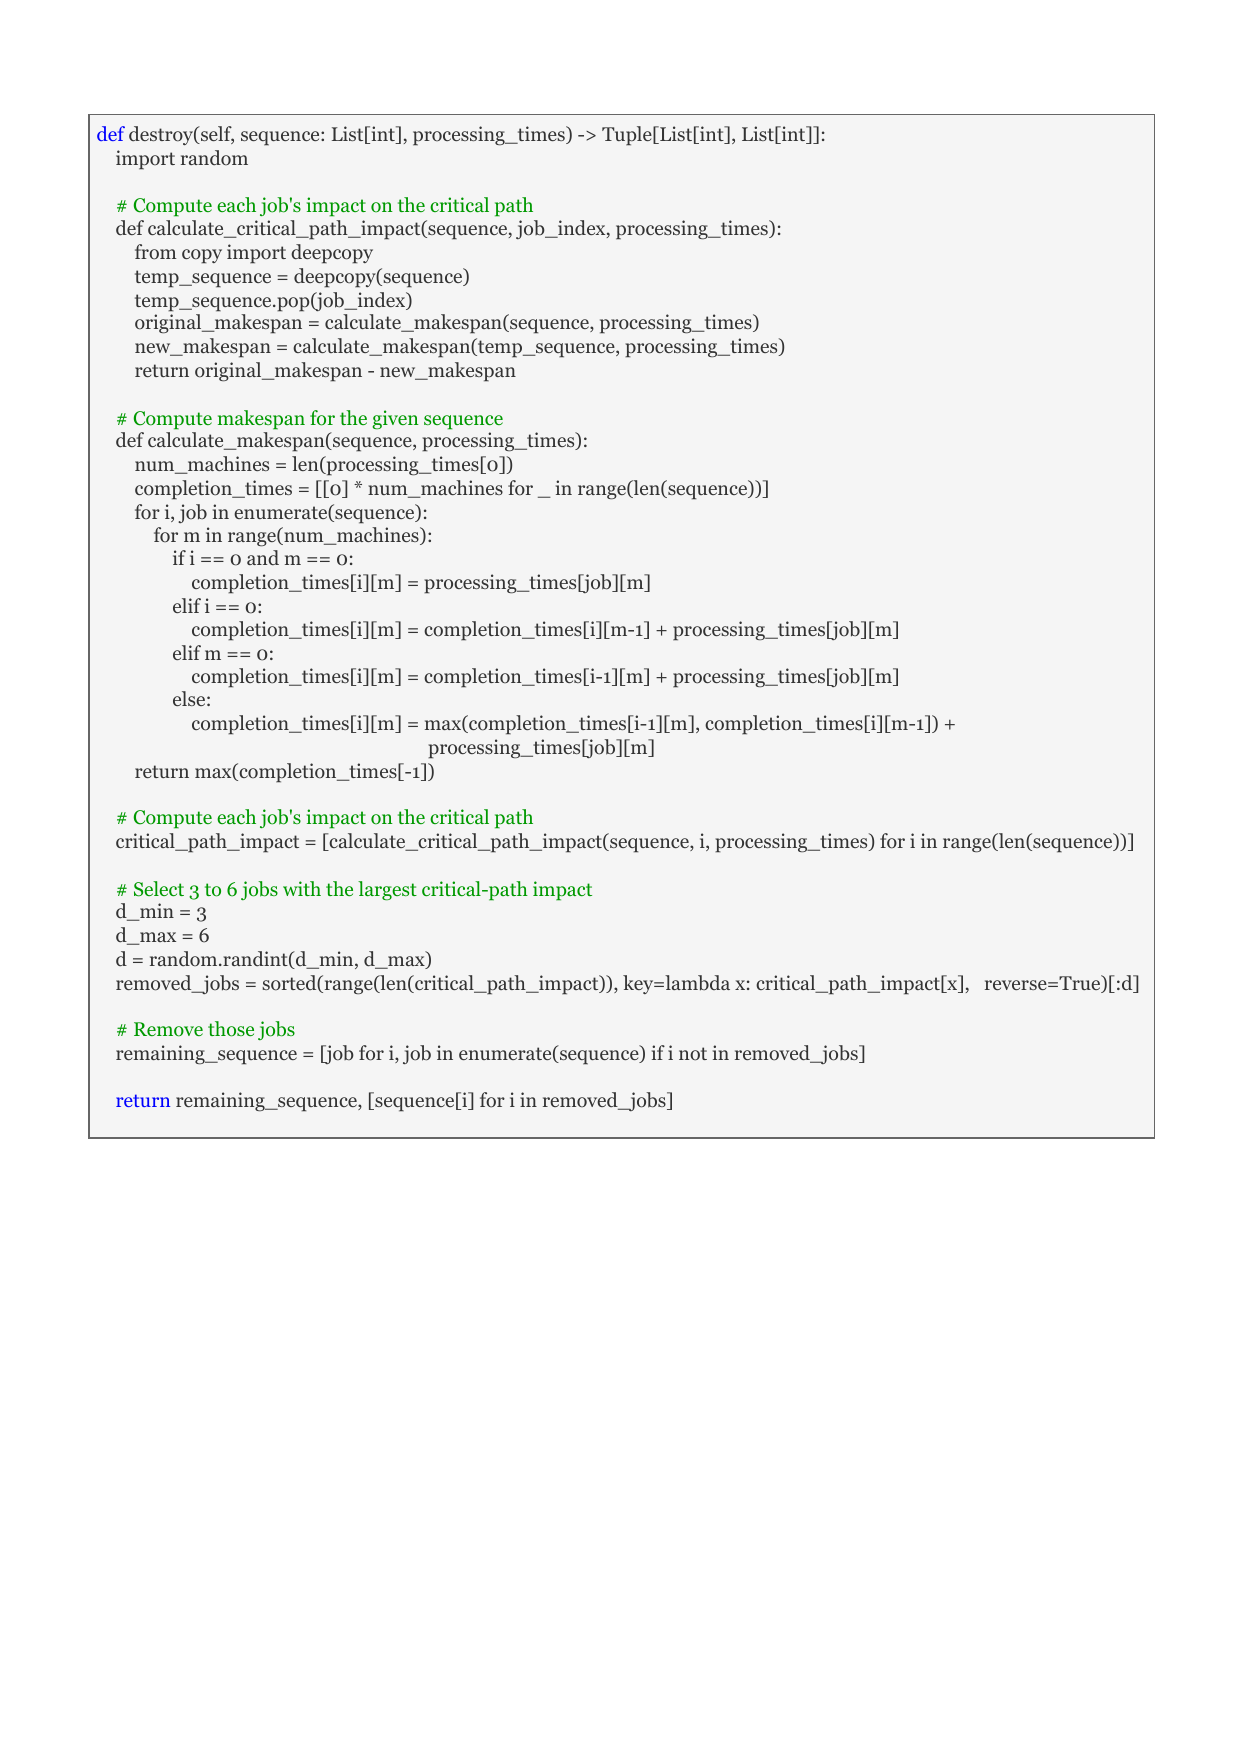}
  \vspace{0.5em}
  \text{Operator2}
\end{center}

\begin{center}
  \includegraphics[width=\linewidth]{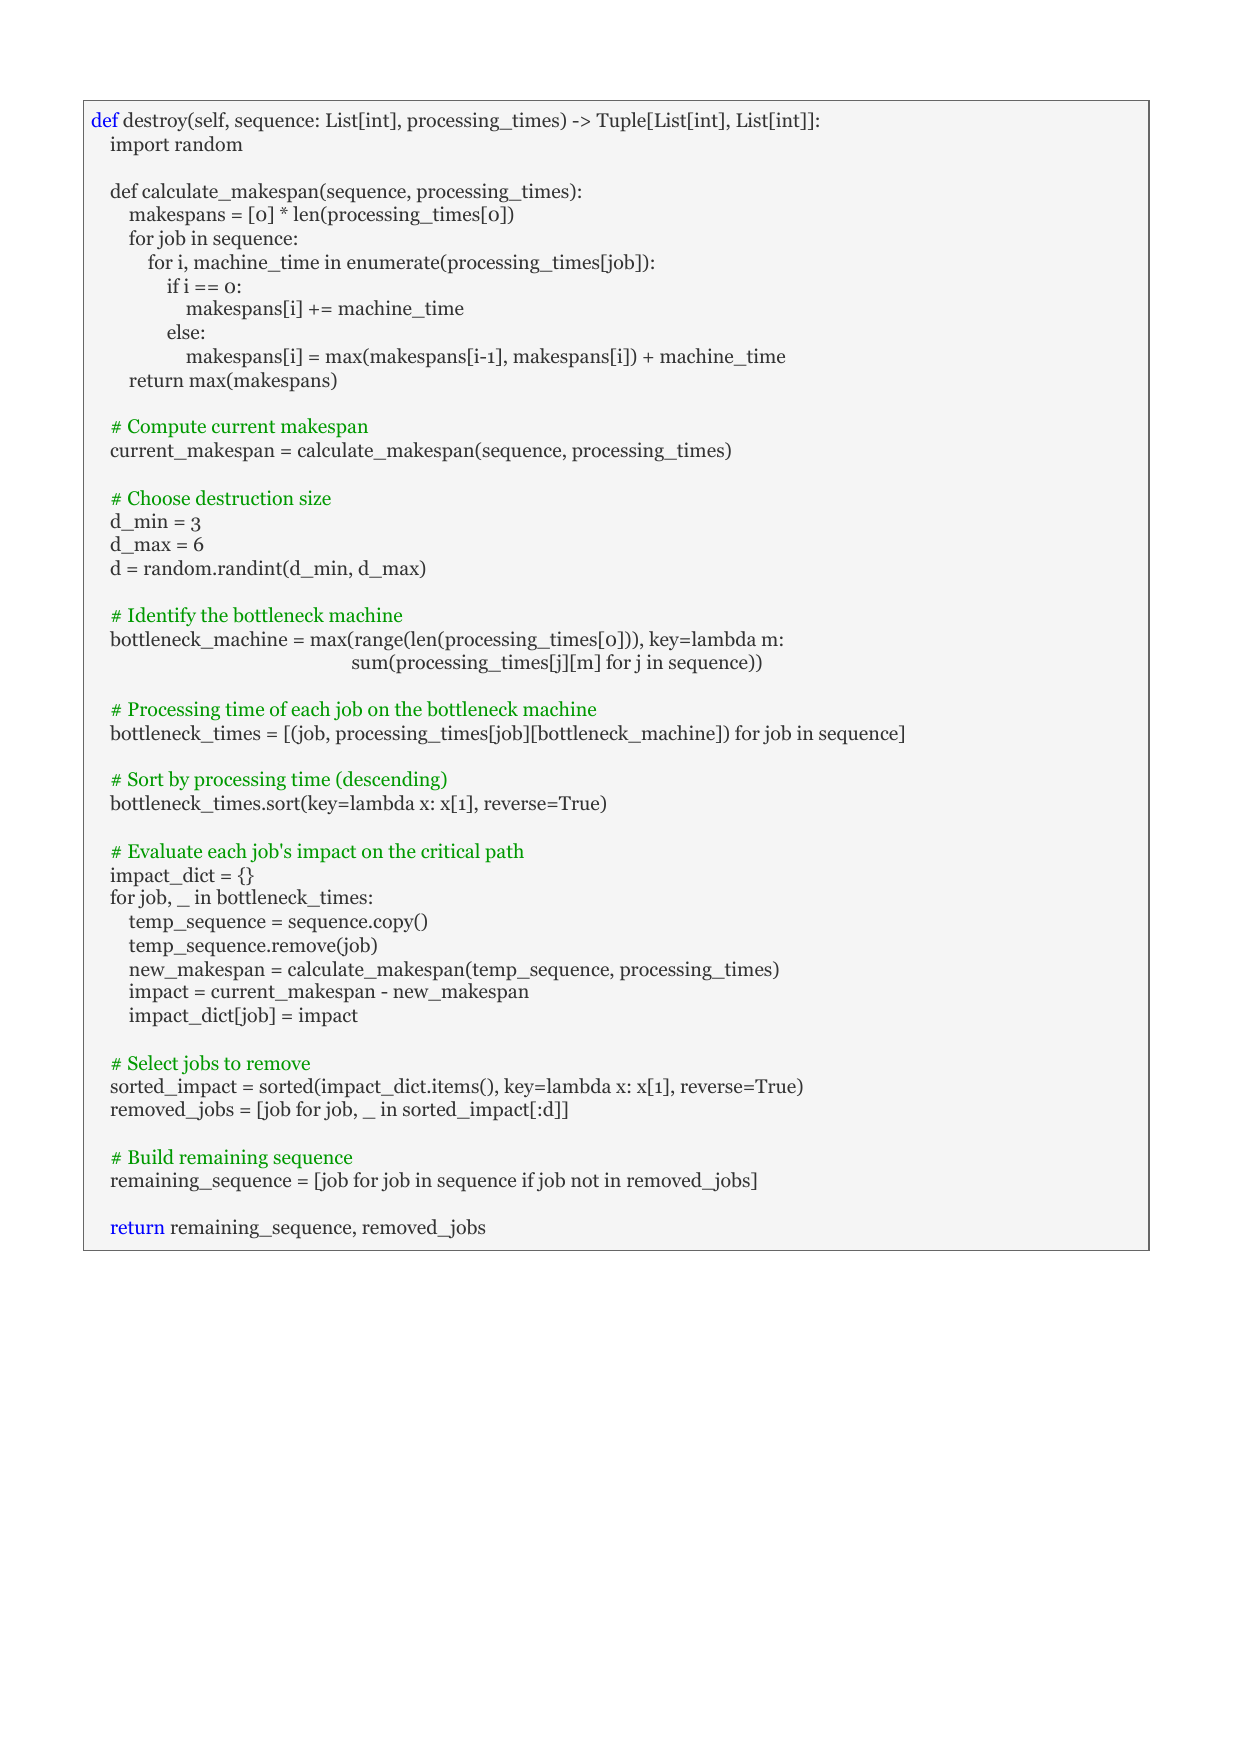}
  \vspace{0.5em}
  \text{Operator3}
\end{center}

\begin{center}
  \includegraphics[width=\linewidth]{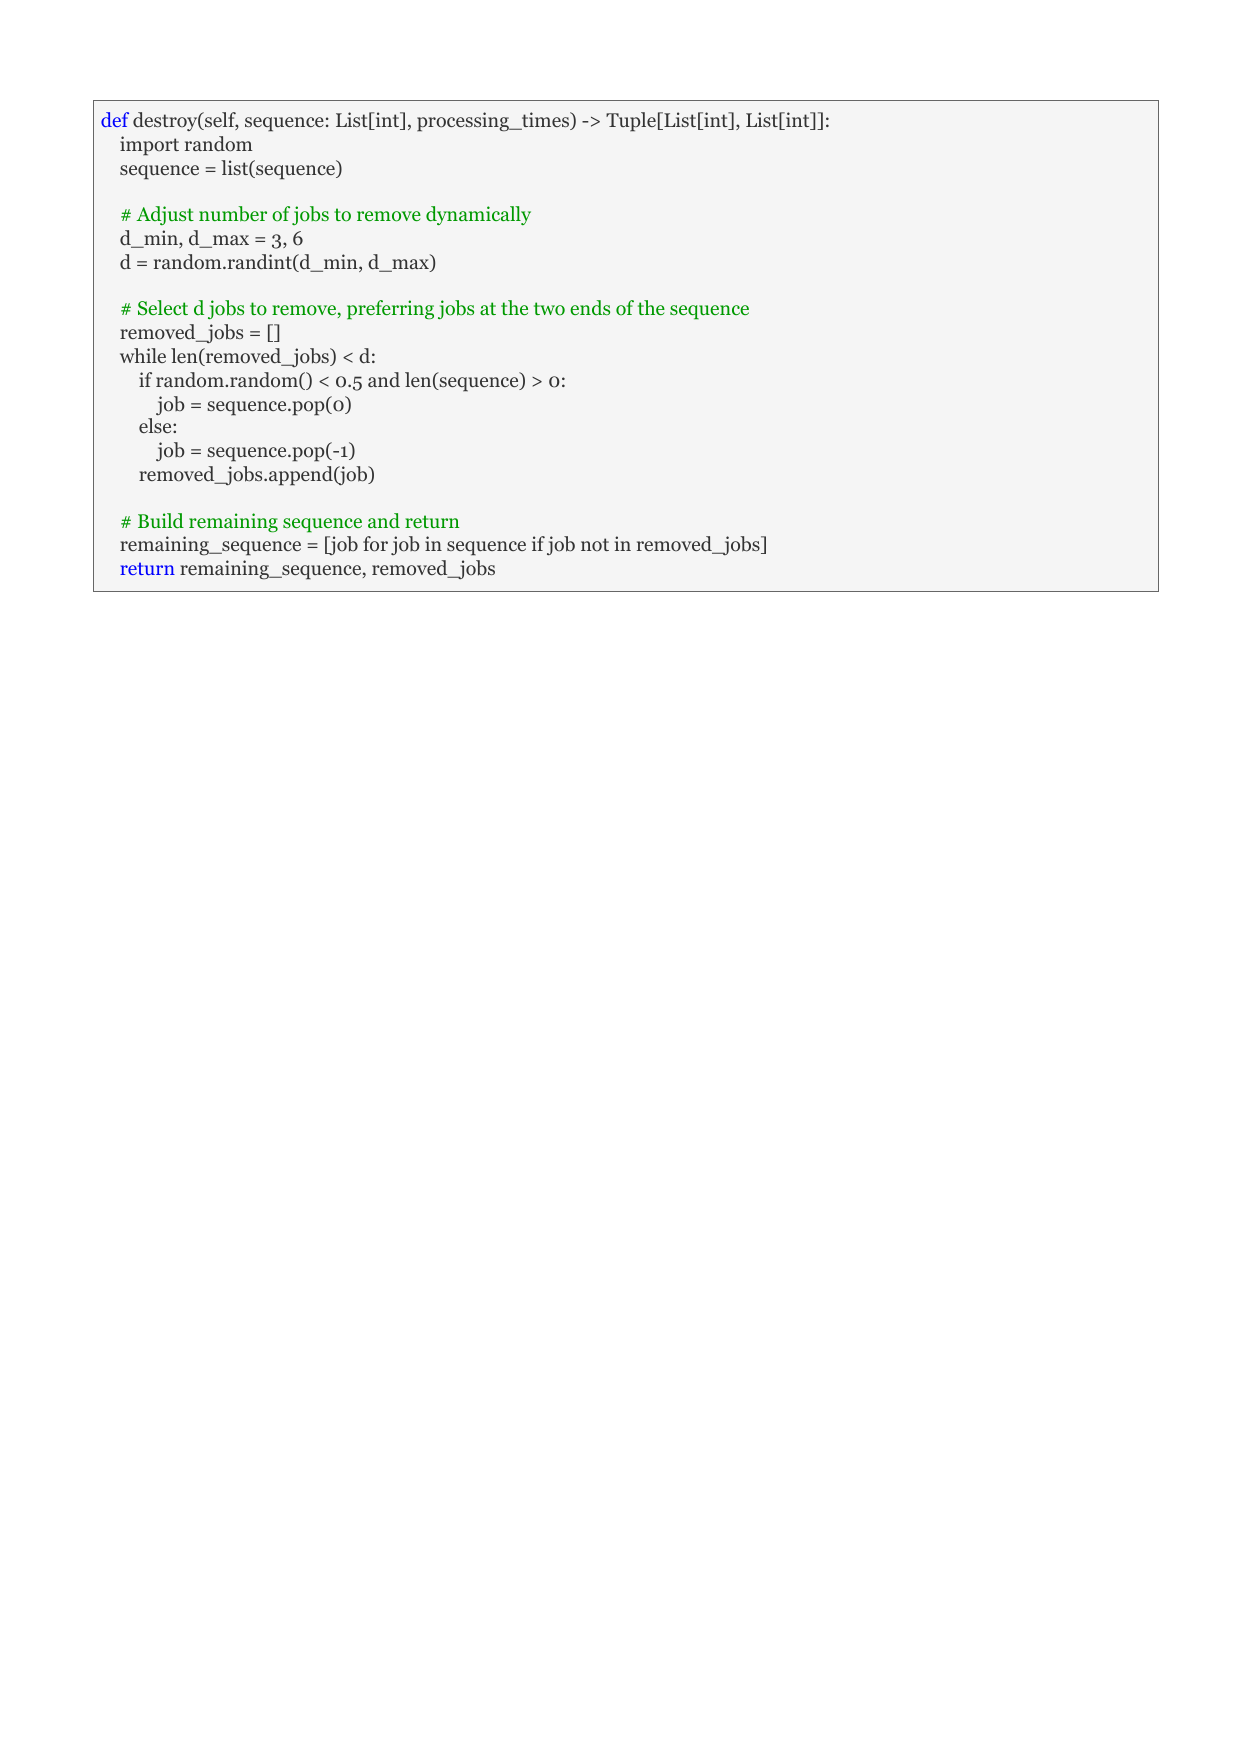}
  \vspace{0.5em}
  \text{Operator4}
\end{center}

\subsection{ReEvo-Style Evolutionary Operations in Co-ReEvo}
\label{supp:reevo_ops}

Co-ReEvo follows the reflective evolutionary cycle of ReEvo in its inner candidate-generation process.
In this cycle, an individual is a code snippet of a heuristic generated by the LLM.
In our implementation, each individual is an executable destruction-operator code snippet that follows the required function signature and can be inserted into the IG-DOE framework.
The main ReEvo-style evolutionary operations in Co-ReEvo are summarized in Table~\ref{tab:reevo_ops}.

\begin{table}[H]
    \centering
    \caption{ReEvo-style evolutionary operations in Co-ReEvo.}
    \label{tab:reevo_ops}
    \begin{tabular}{p{0.24\linewidth}|p{0.68\linewidth}}
        \toprule
        Operation & Implementation in Co-ReEvo \\
        \midrule
        Individual encoding
        & Following ReEvo, each individual is represented as a code snippet generated by the LLM, without a predefined encoding format except for the specified function signature. In Co-ReEvo, the code snippet implements a destruction operator that returns the jobs to be removed in the destruction phase. \\
        \hline
        Population initialization
        & The generator LLM initializes a population using the task specification, including the PFSP description, heuristic designation and functionality, the required function interface, optional seed operators, domain knowledge, and the current DOE state. \\
        \hline
        Candidate evaluation
        & As in ReEvo, generated candidates are evaluated after initialization, crossover, and mutation. In Co-ReEvo, the original standalone evaluation objective is replaced by a cooperative performance value, which is computed after appending the candidate to the current ensemble. \\
        \hline
        Selection
        & Parent pairs are sampled from successfully executed candidate operators, while avoiding pairs with identical cooperative fitness values when possible. \\
        \hline
        Short-term reflection
        & For each parent pair, the reflector LLM performs a comparative analysis based on their relative cooperative performance and gives hints for improved operator design. These short-term reflections provide local guidance for crossover. \\
        \hline
        Crossover
        & The generator LLM creates offspring operators using the task specification, a pair of parent operator codes, explicit indications of their relative performance, short-term reflections over the pair, generation instructions, and the current DOE state. \\
        \hline
        Long-term reflection
        & The reflector LLM summarizes previous long-term reflections and newly gained short-term reflections into accumulated design hints for improving future operators. \\
        \hline
        Elitist mutation
        & Based on long-term reflections, the generator LLM samples new operators to improve the current elite operator. The mutation prompt uses the task specification, the elite operator, long-term reflections, generation instructions, and the current DOE state. \\
        \hline
        Invalid-candidate filtering
        & Operators with syntax errors or runtime failures are excluded from the set of successfully executed candidates and therefore cannot be selected as parents or elites. \\
        \bottomrule
    \end{tabular}
\end{table}

The main difference from the original single-heuristic ReEvo setting lies in the evaluation objective.
Original ReEvo evolves a standalone heuristic according to its individual performance.
By contrast, Co-ReEvo evaluates each candidate after temporarily appending it to the current DOE.
Therefore, selection, crossover, and elitist mutation are guided by the performance of the enlarged ensemble formed by the candidate and the current DOE, rather than by the candidate's standalone performance alone.
The additional DOE state-awareness prompt further encourages the LLM to generate operators that complement the operators already included in the ensemble.

\subsection{Complete Results on Industrial-Data-Derived Instances}
\label{supp:industrial_boxplot}

\begin{figure}[H]
  \centering
  \includegraphics[width=0.9\linewidth]{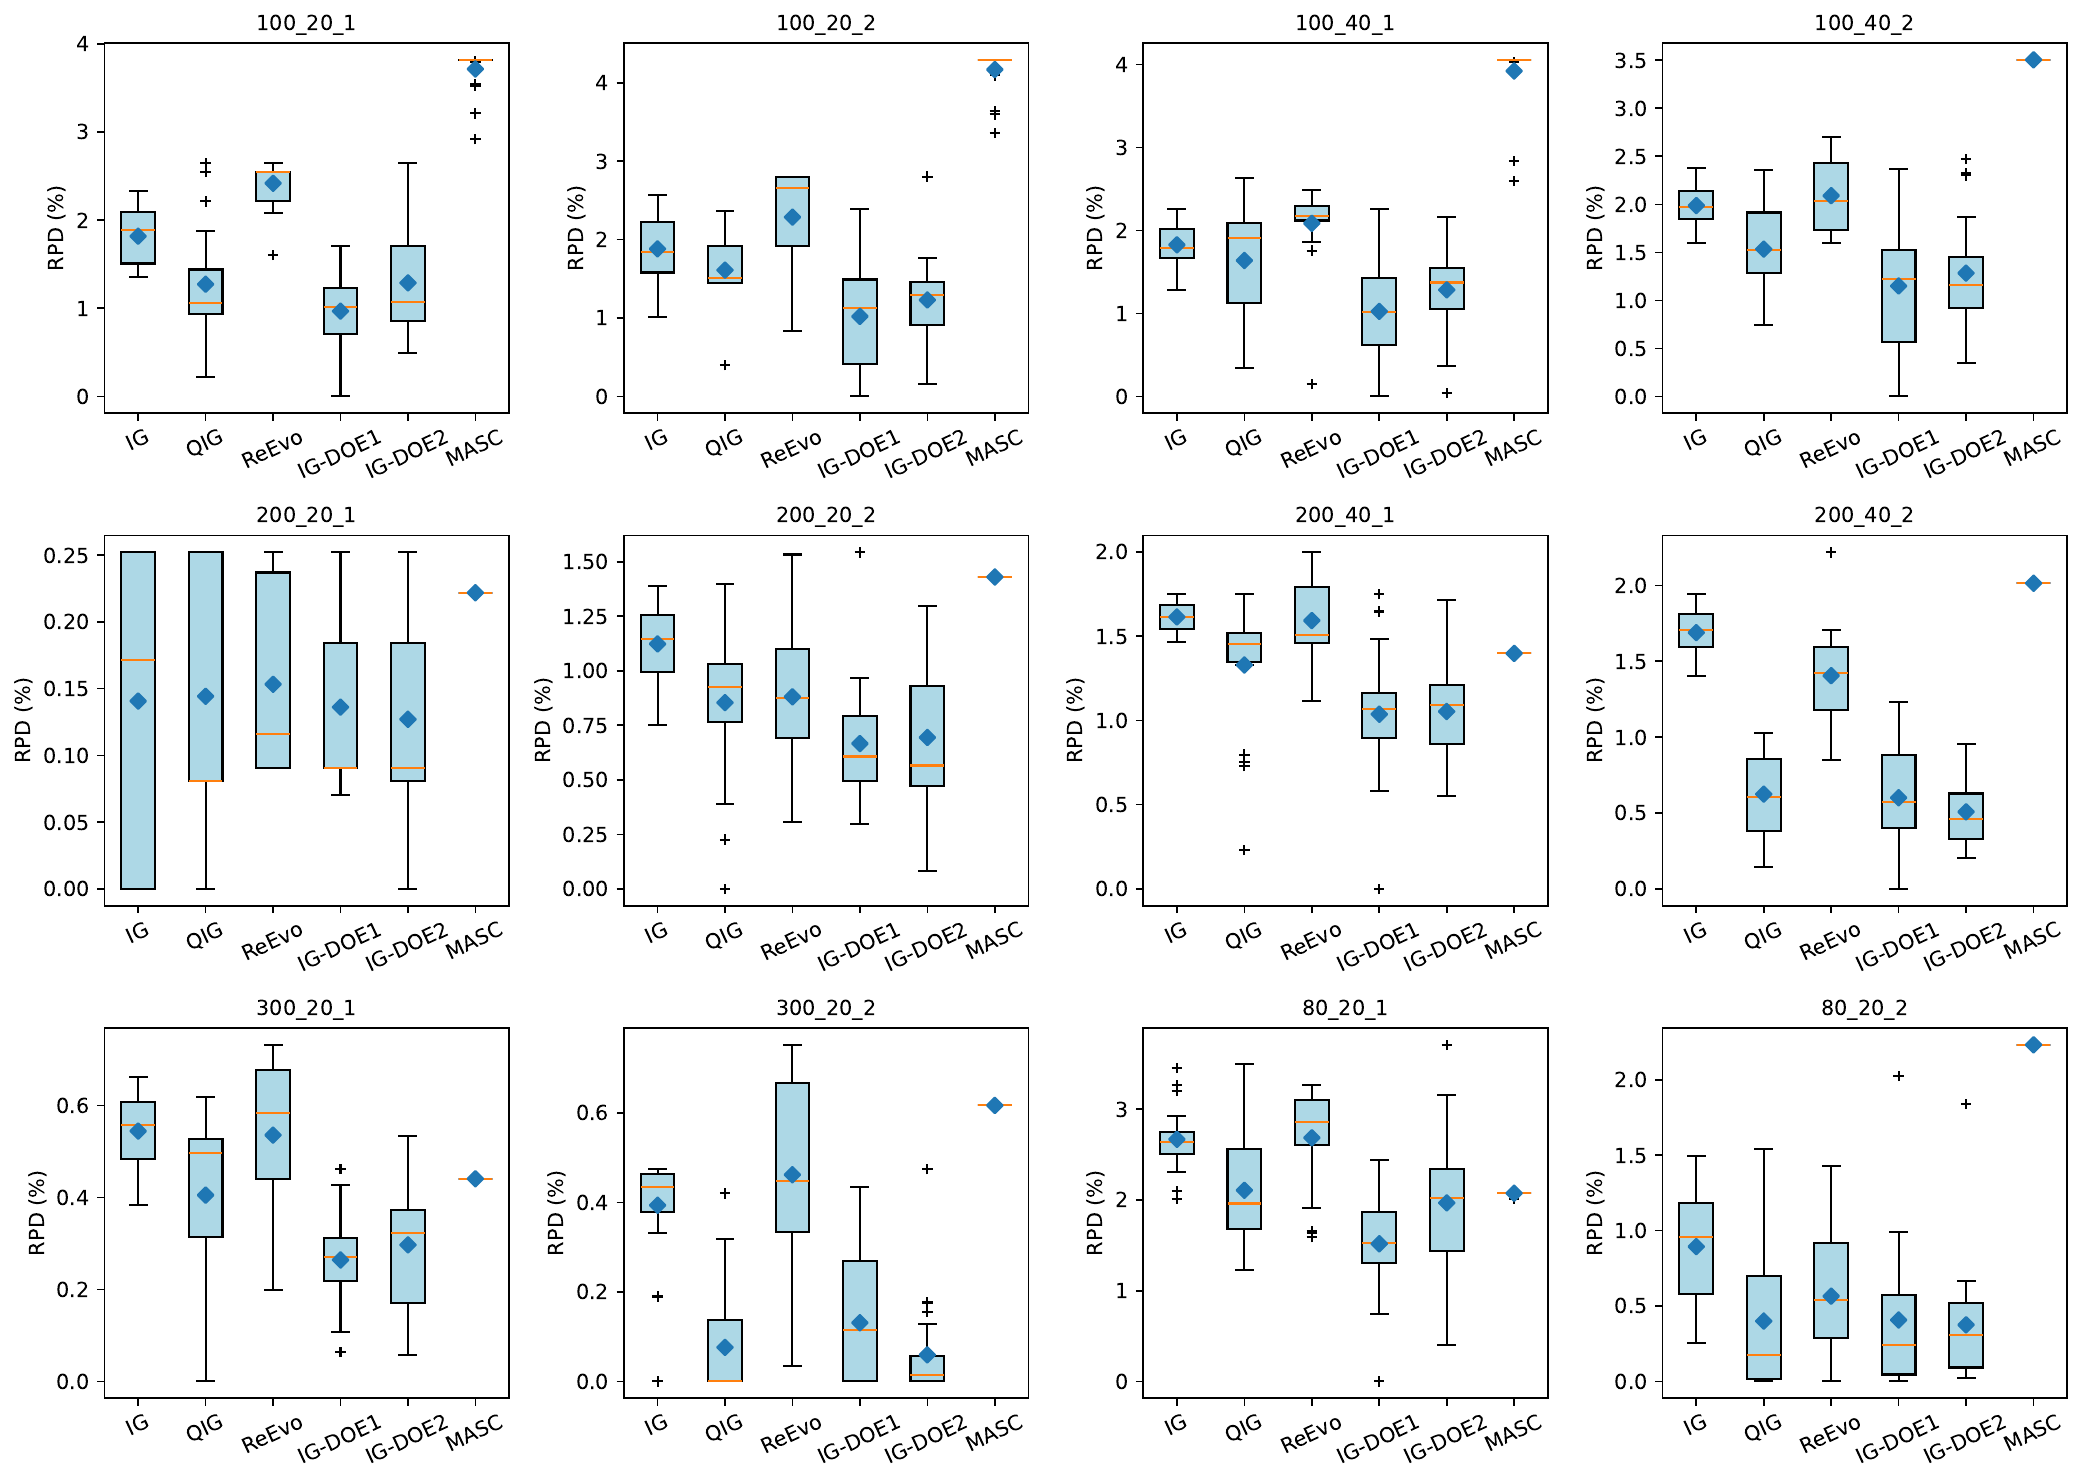}
  \caption{Complete distributions of run-level RPD values of all compared algorithms, including MASC, on the 12 industrial-data-derived PFSP instances.}
  \label{fig:supp_real_data_masc}
\end{figure}

\end{document}
